# Supplementary material for: Gas phase metallicity determinations in nearby AGNs with SDSS-IV MaNGA: evidence of metal poor accretion
Source: arXiv:2203.08602 source file (2022-03-16)
Supplement: Supplementary file 1 [file supplementary_figures.pdf]

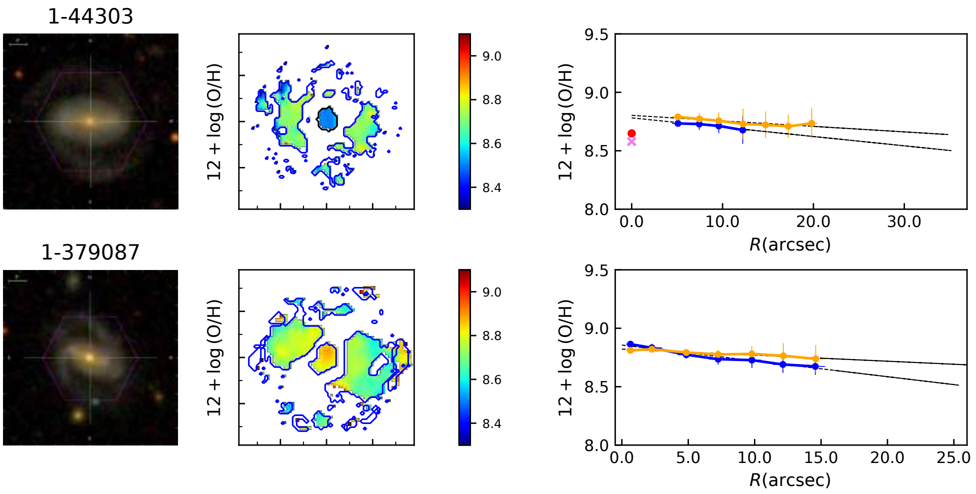


**Figure A1.** As Fig 3 but for the AGN host 1-44303.

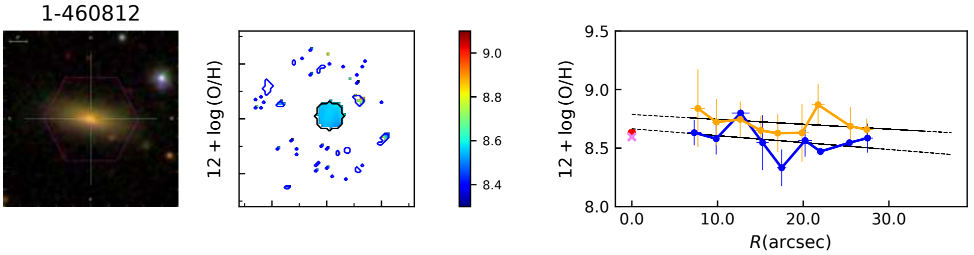


**Figure A2.** As Fig 3 but for the AGN host 1-460812.

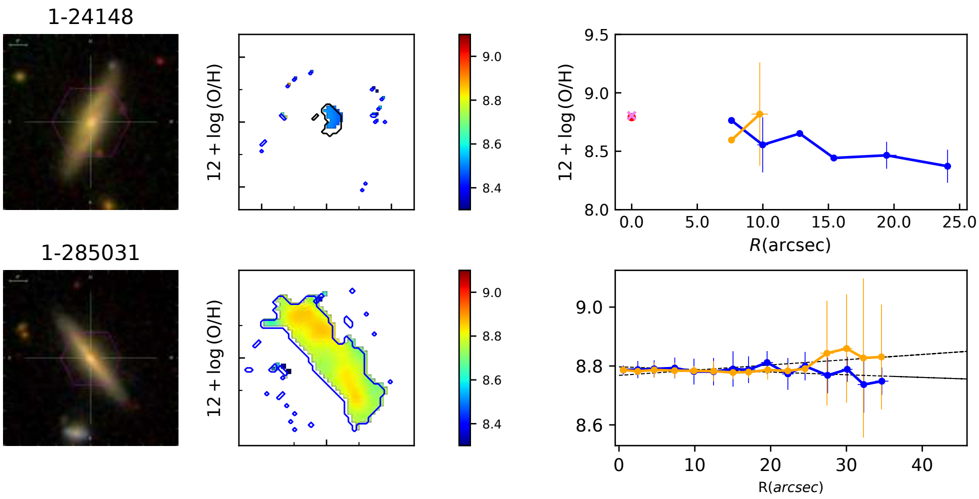


**Figure A3.** As Fig 3 but for the AGN host 1-24148.

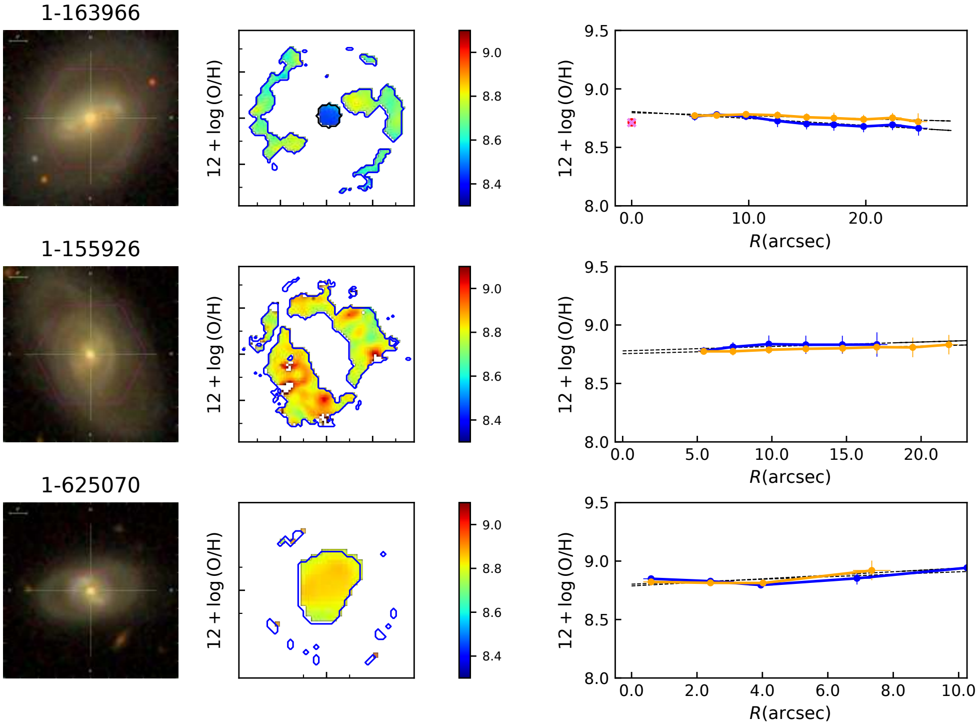


**Figure A4.** As Fig 3 but for the AGN host 1-163966.

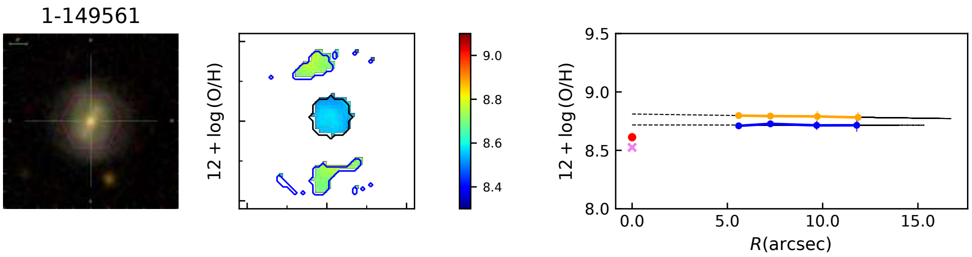


**Figure A5.** As Fig 3 but for the AGN host 1-149561.

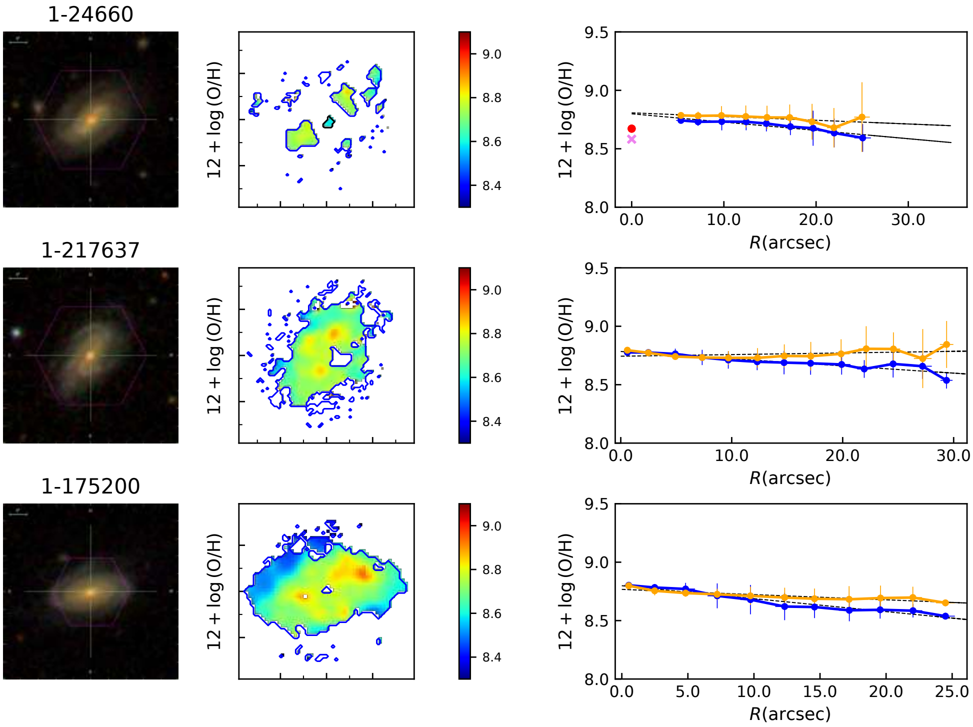


**Figure A6.** As Fig 3 but for the AGN host 1-24660.

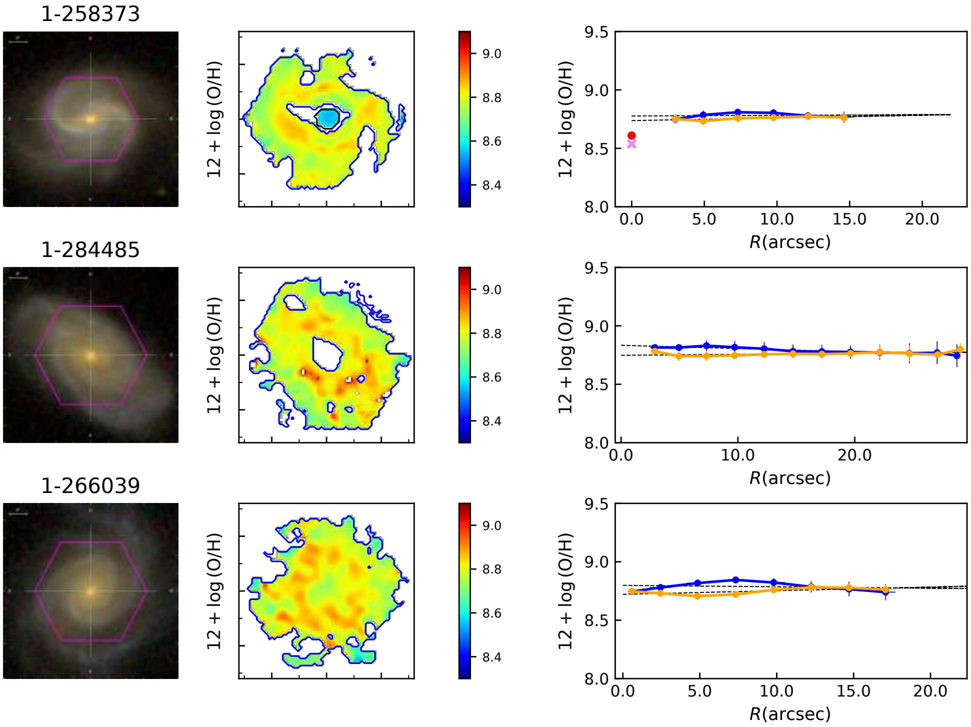


**Figure A7.** As Fig 3 but for the AGN host 1-258373.

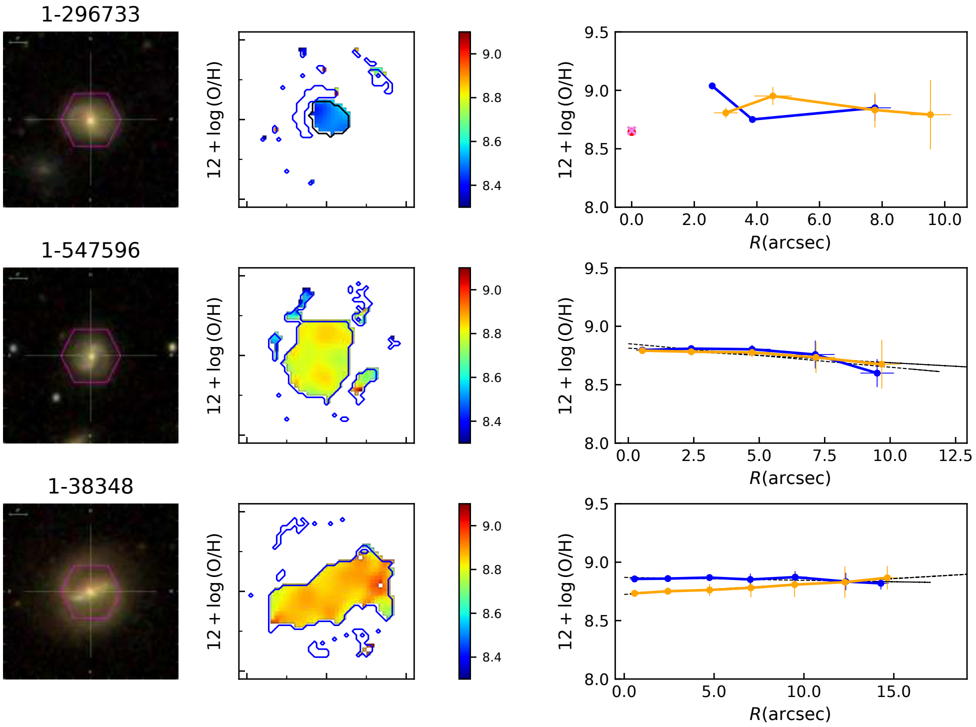


**Figure A8.** As Fig 3 but for the AGN host 1-296733.

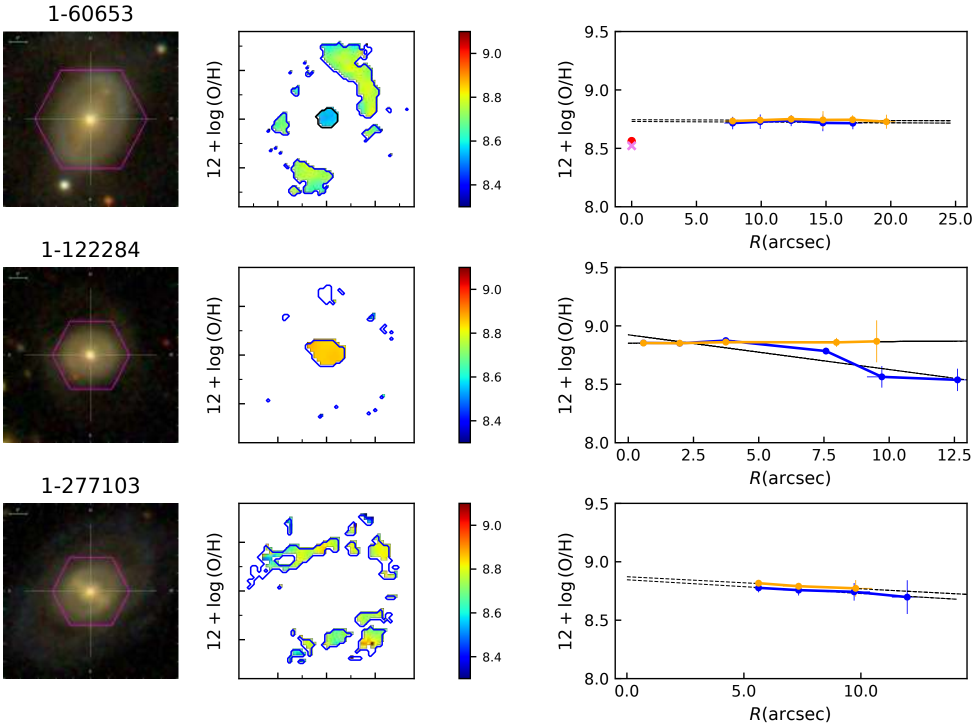


**Figure A9.** As Fig 3 but for the AGN host 1-60653.

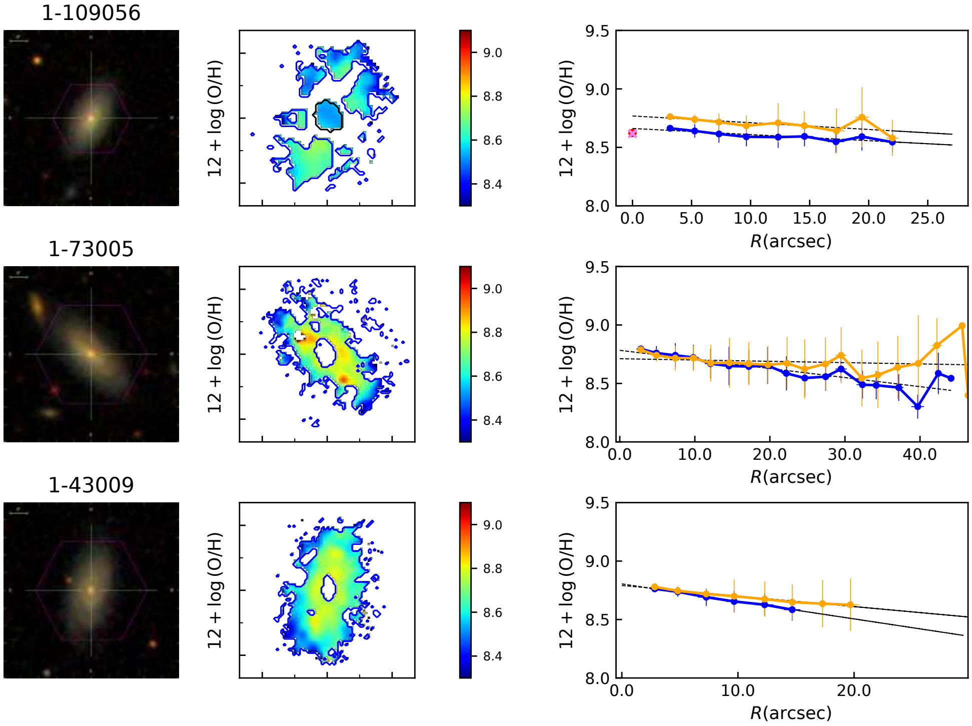


**Figure A10.** As Fig 3 but for the AGN host 1-109056.

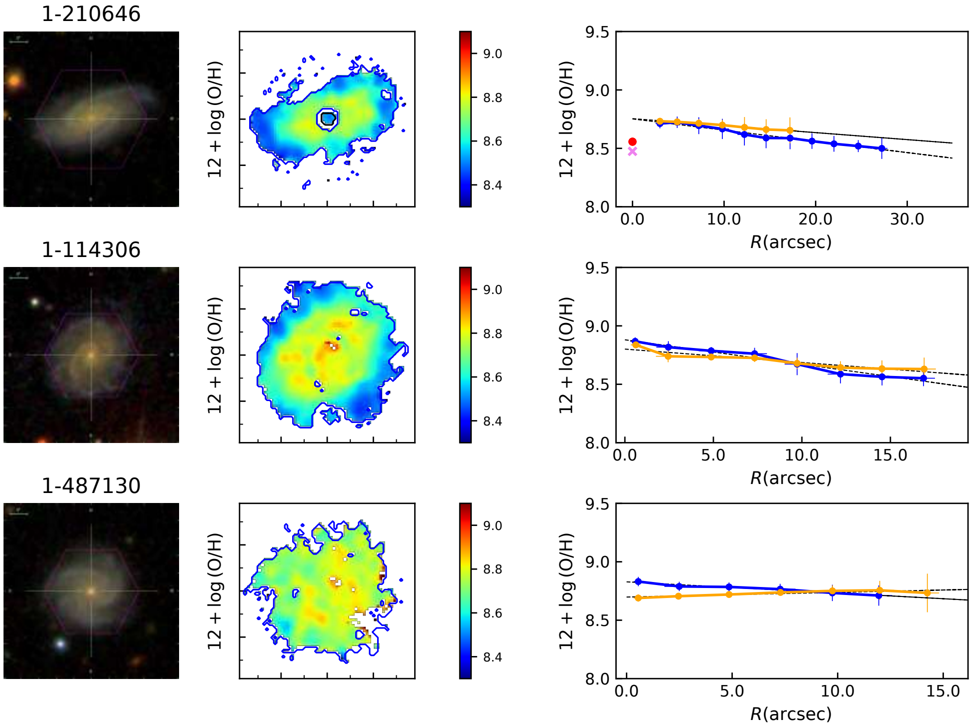


**Figure A11.** As Fig 3 but for the AGN host 1-210646.

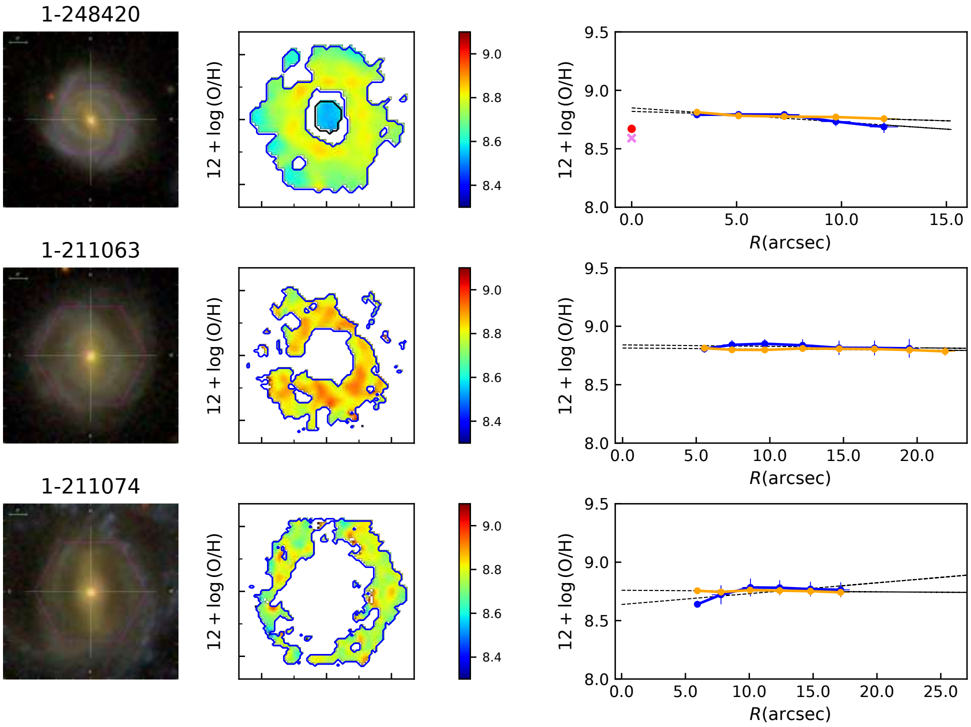


**Figure A12.** As Fig 3 but for the AGN host 1-248420.

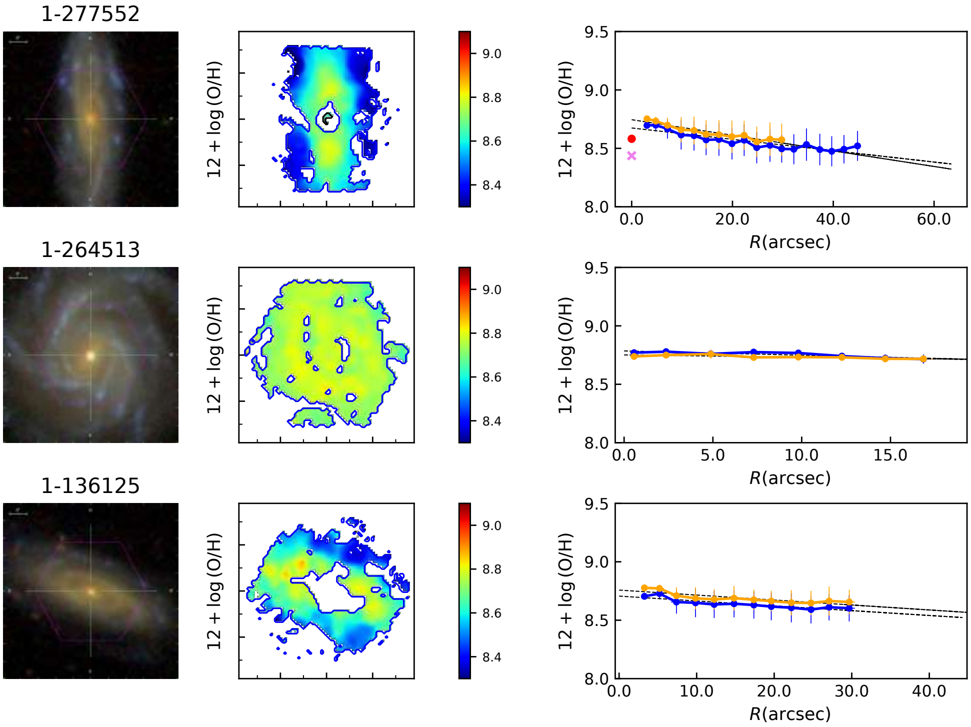


**Figure A13.** As Fig 3 but for the AGN host 1-277552.

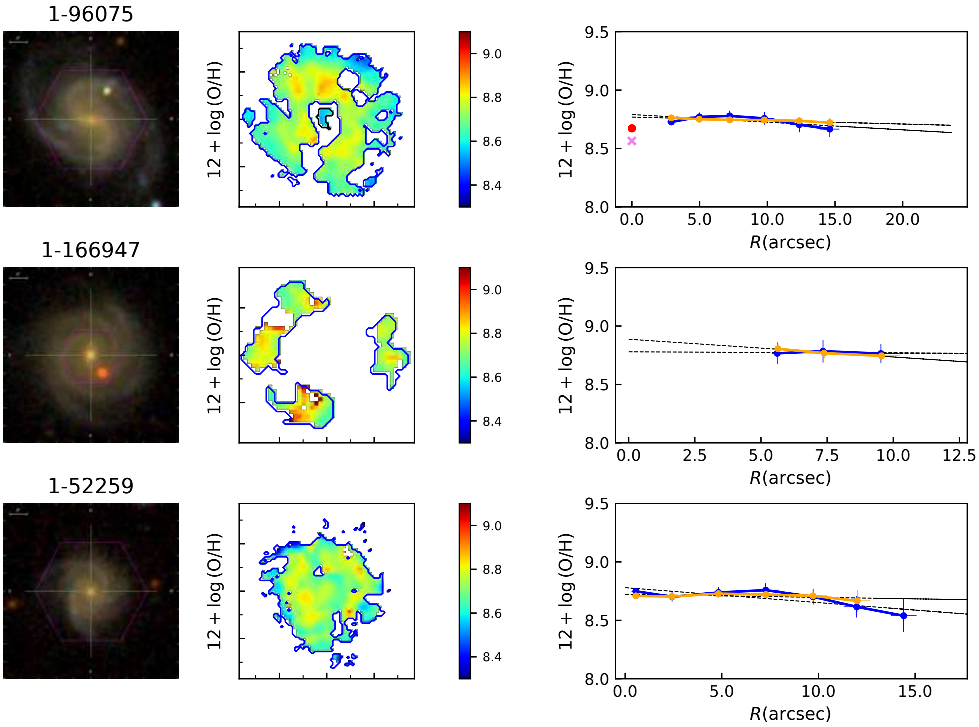


**Figure A14.** As Fig 3 but for the AGN host 1-96075.

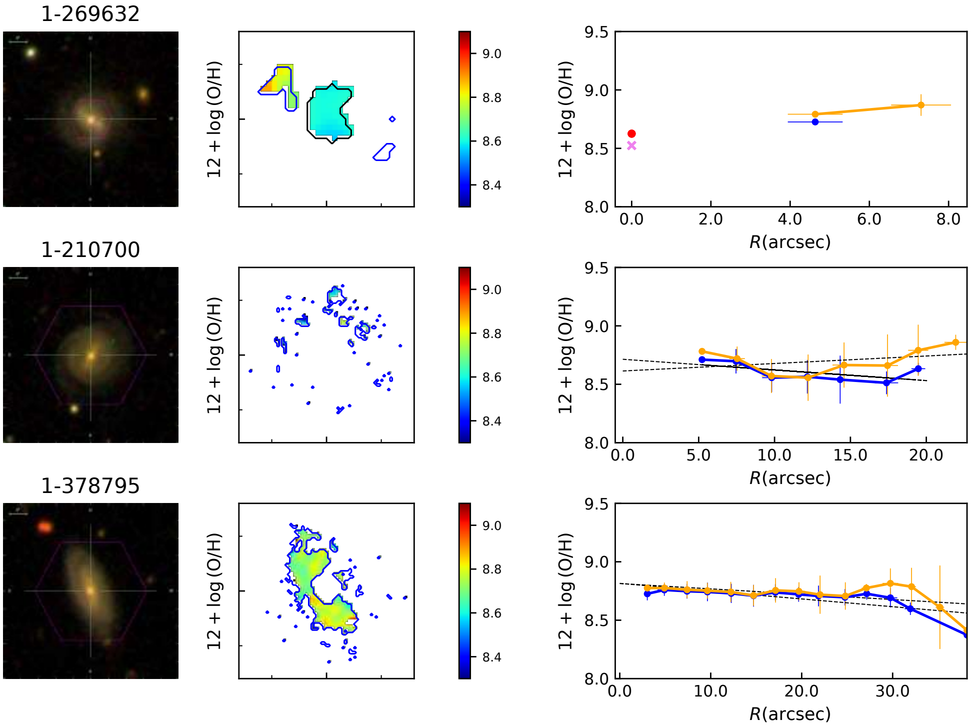


**Figure A15.** As Fig 3 but for the AGN host 1-269632.

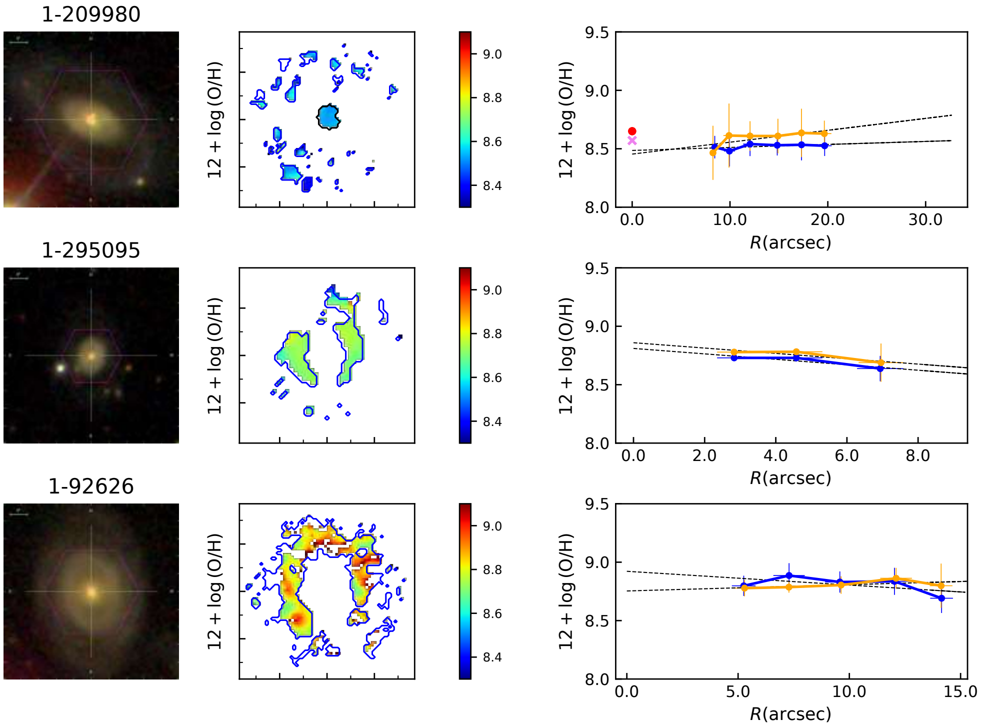


**Figure A16.** As Fig 3 but for the AGN host 1-209980.

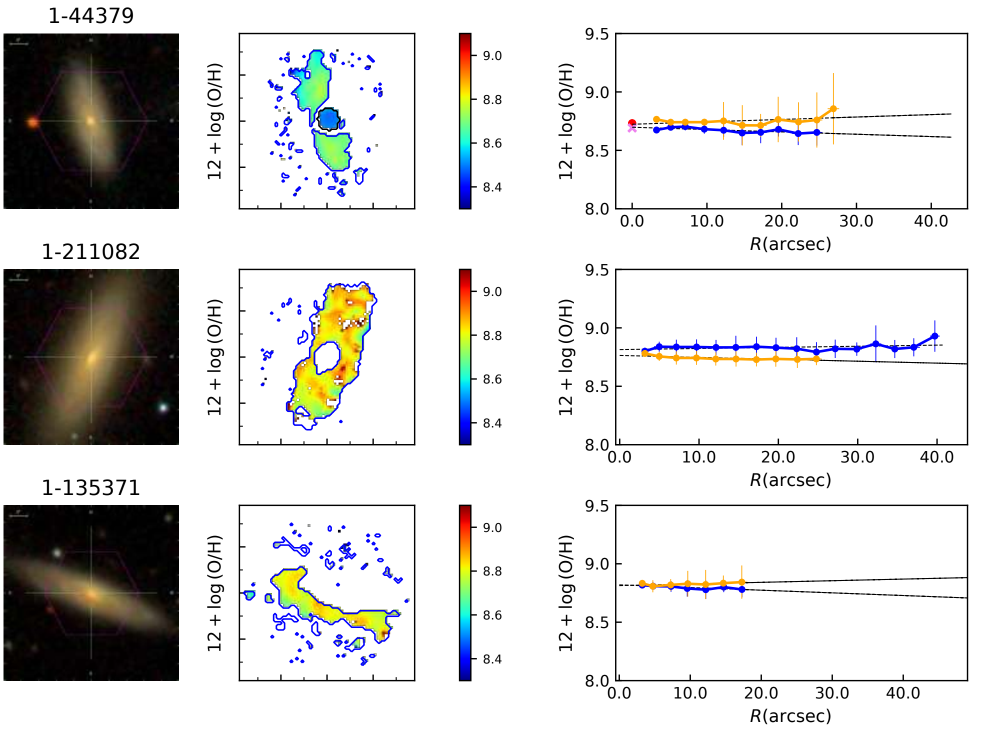


**Figure A17.** As Fig 3 but for the AGN host 1-44379.

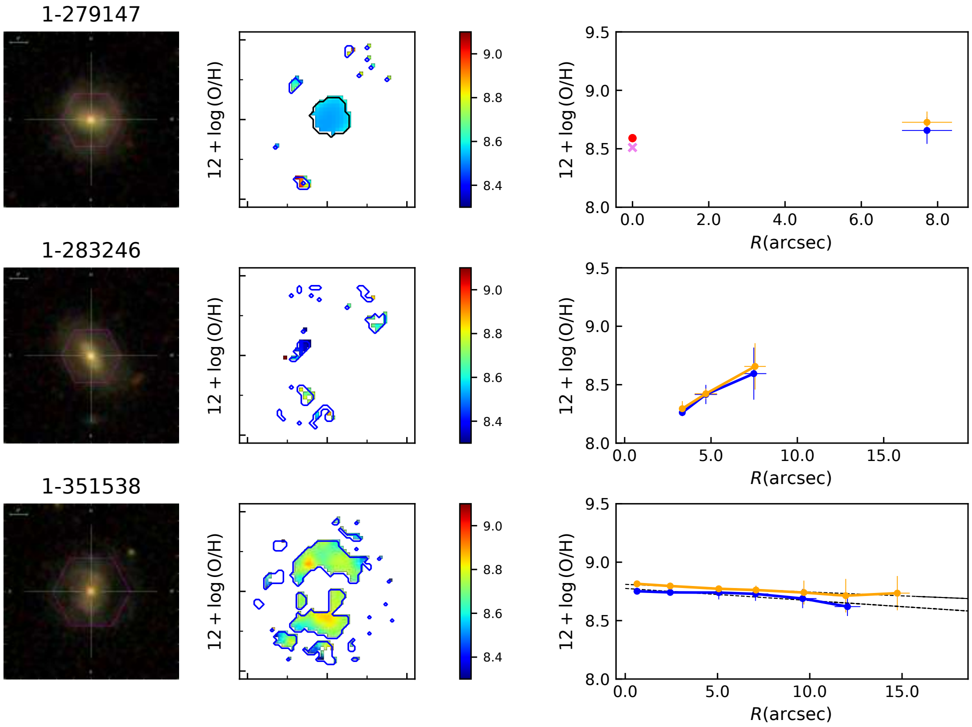


**Figure A18.** As Fig 3 but for the AGN host 1-279147.

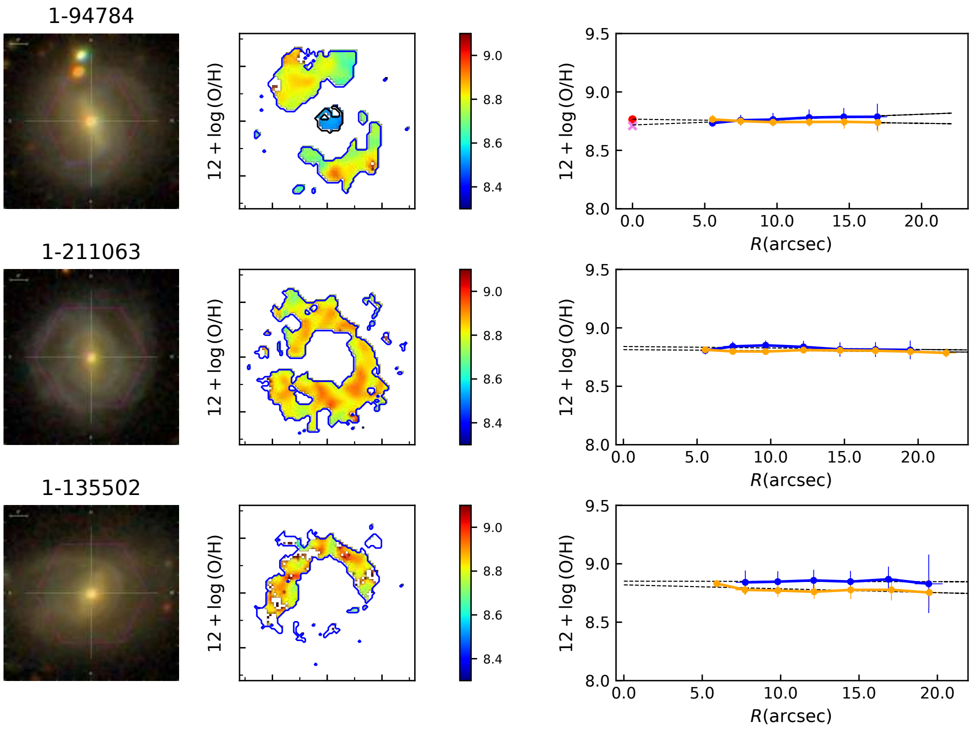


**Figure A19.** As Fig 3 but for the AGN host 1-94784.

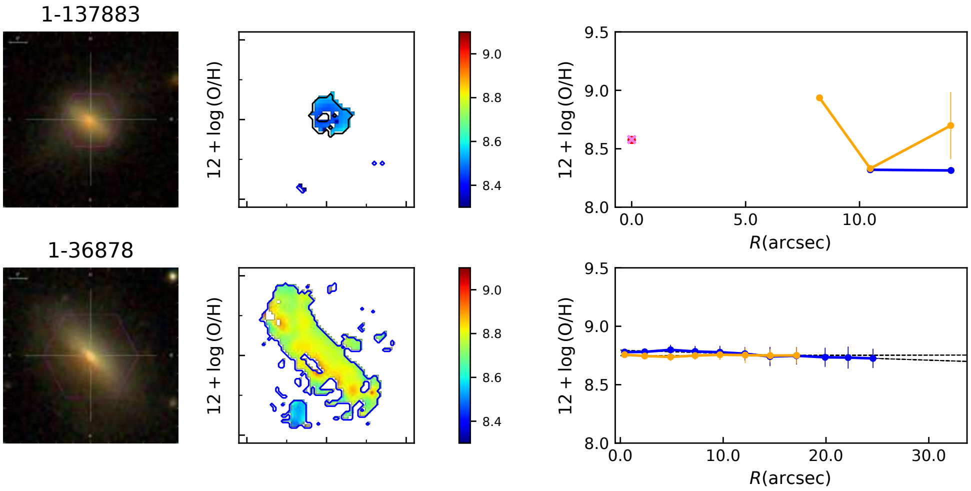


**Figure A20.** As Fig 3 but for the AGN host 1-137883.

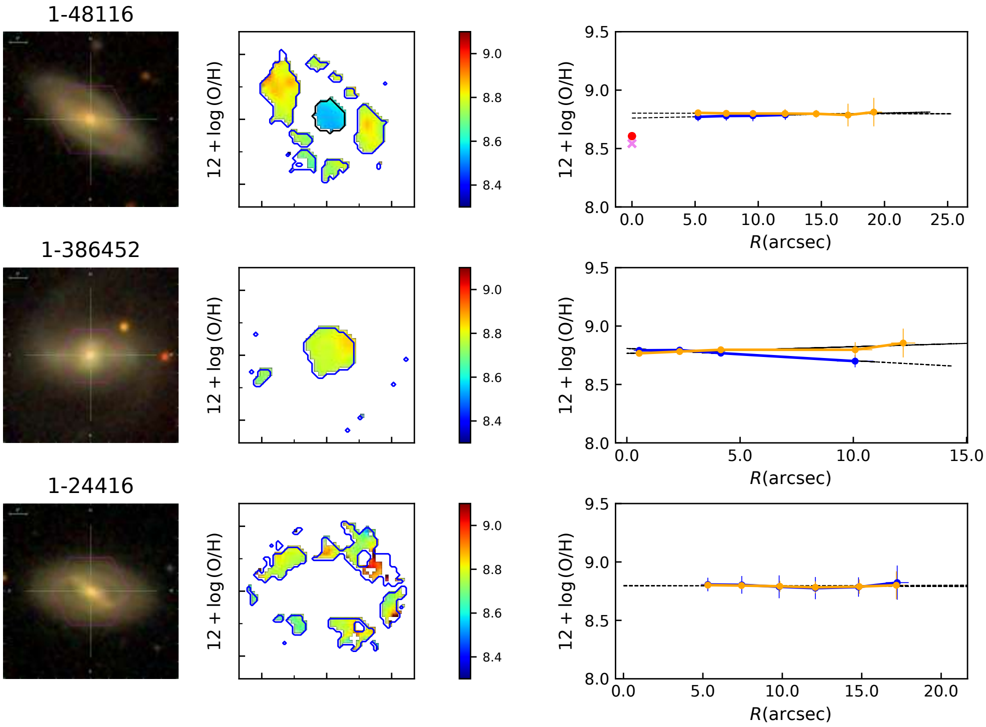


**Figure A21.** As Fig 3 but for the AGN host 1-48116.

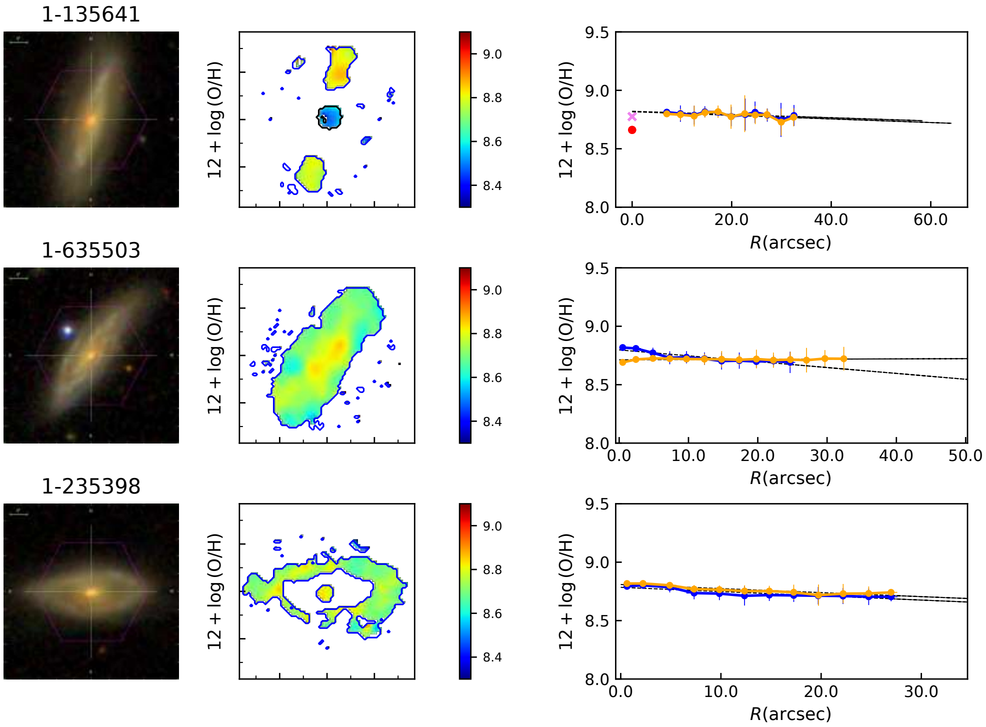


**Figure A22.** As Fig 3 but for the AGN host 1-135641.

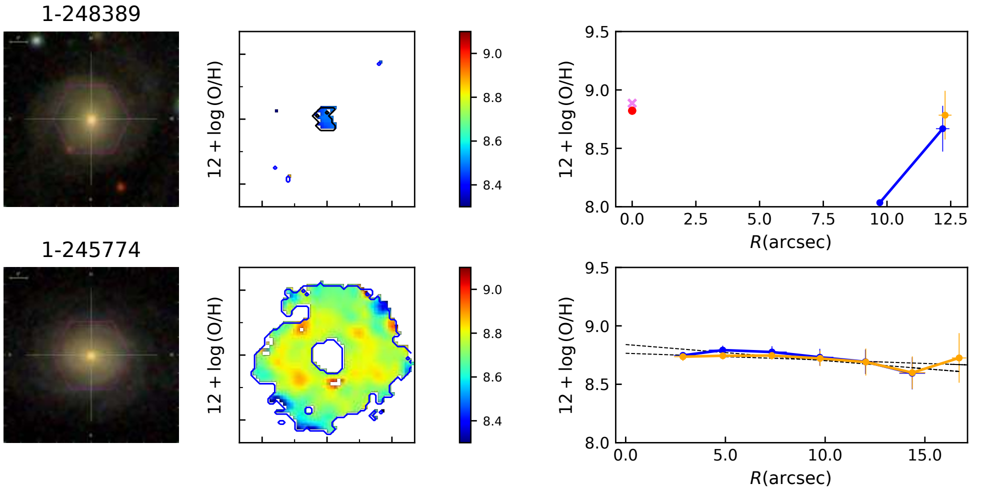


**Figure A23.** As Fig 3 but for the AGN host 1-248389.

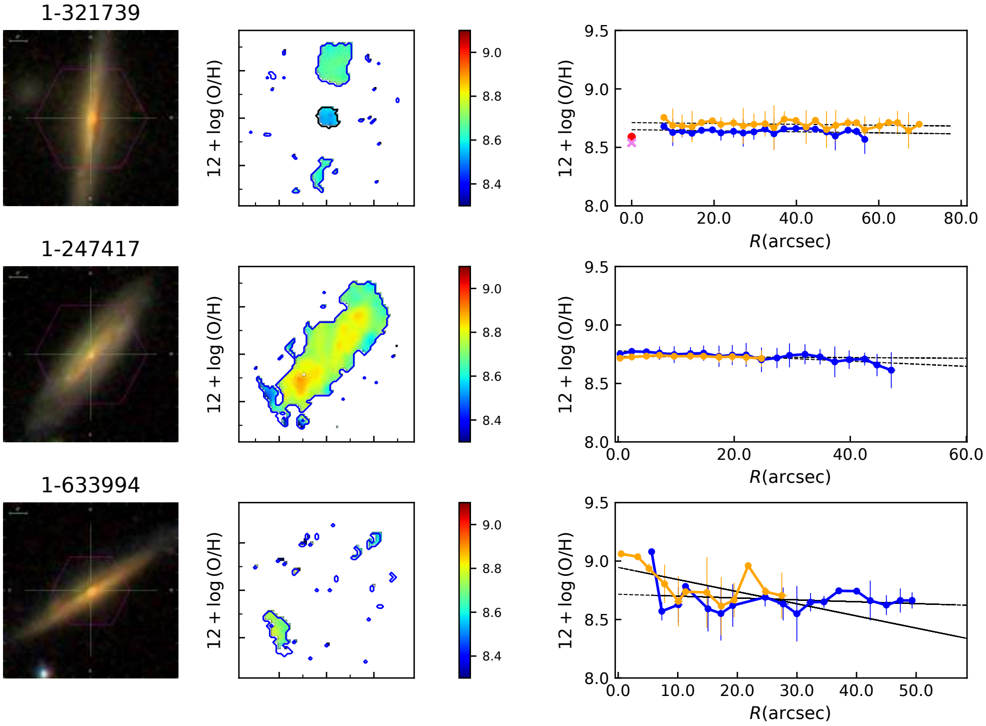


**Figure A24.** As Fig 3 but for the AGN host 1-321739.

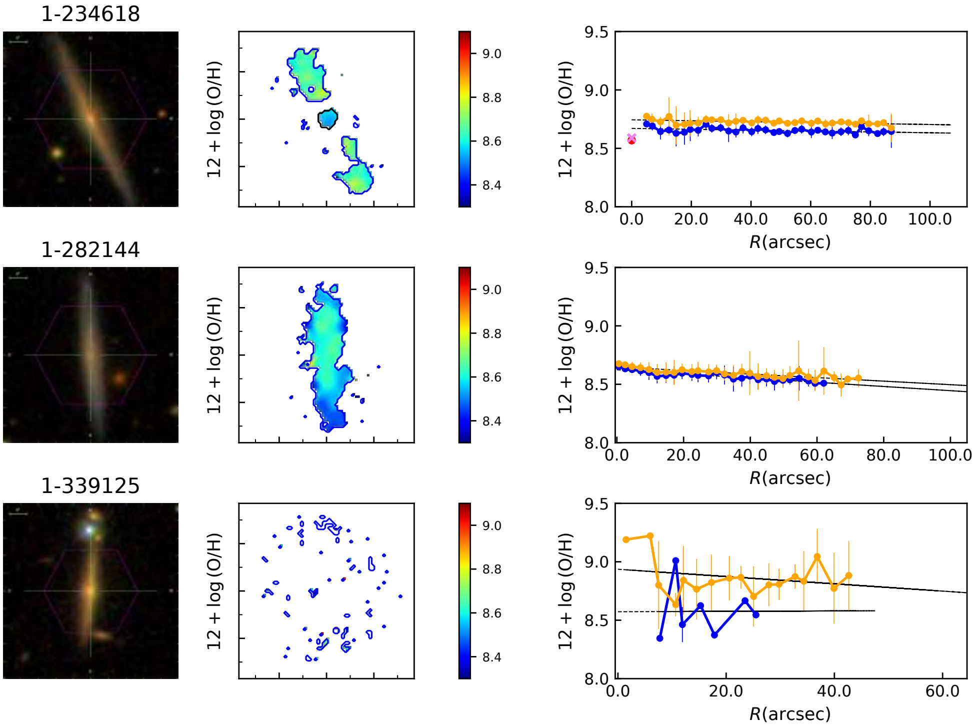


**Figure A25.** As Fig 3 but for the AGN host 1-234618.

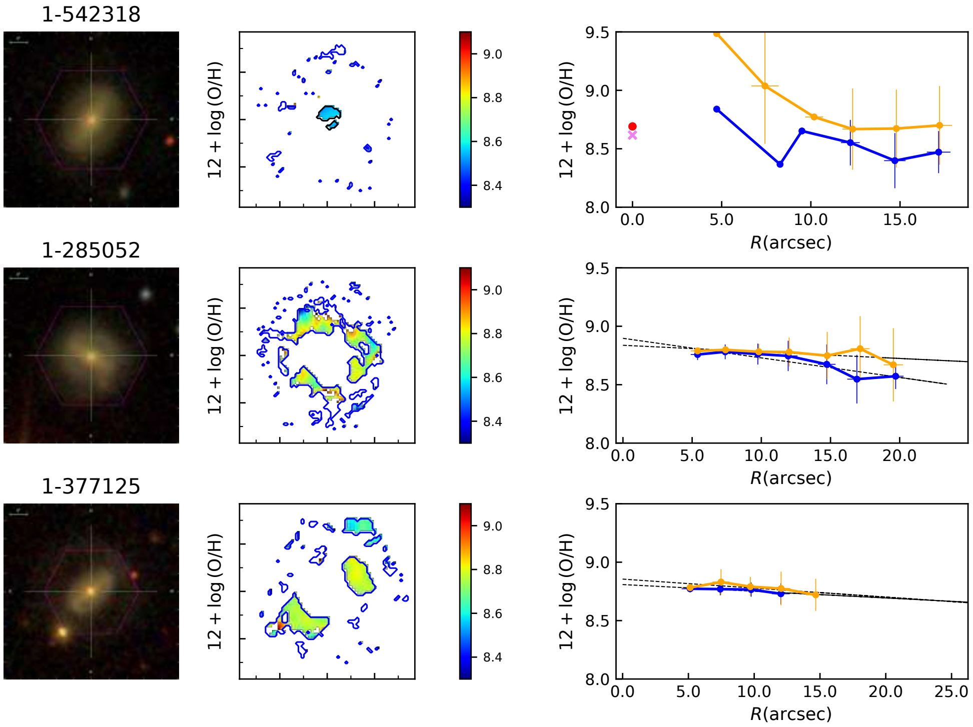


**Figure A26.** As Fig 3 but for the AGN host 1-542318.

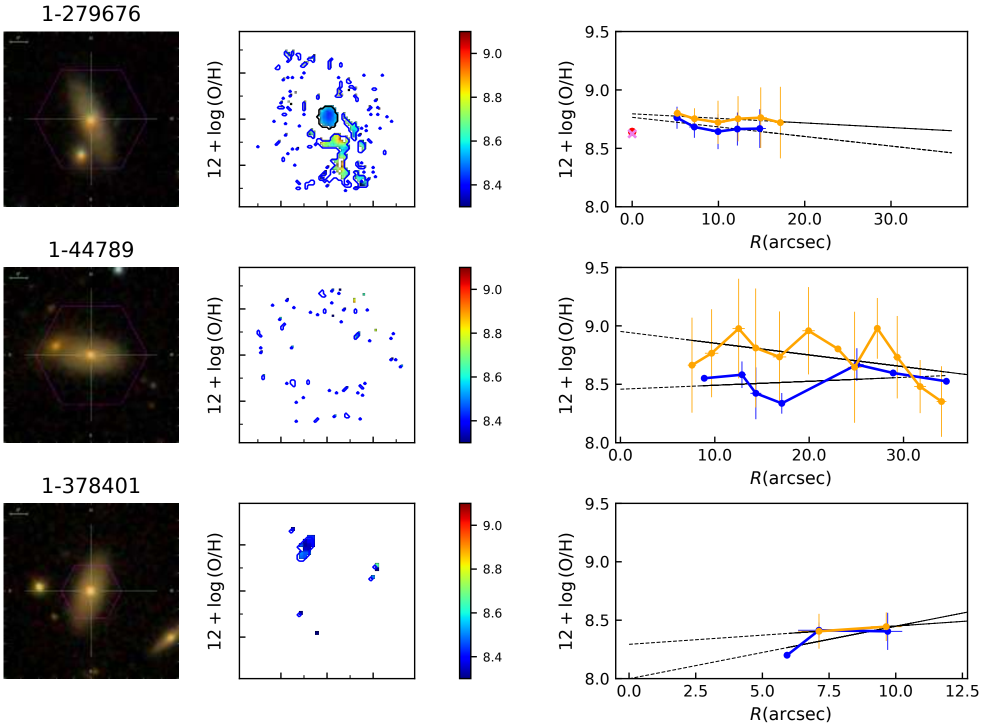


**Figure A27.** As Fig 3 but for the AGN host 1-279676.

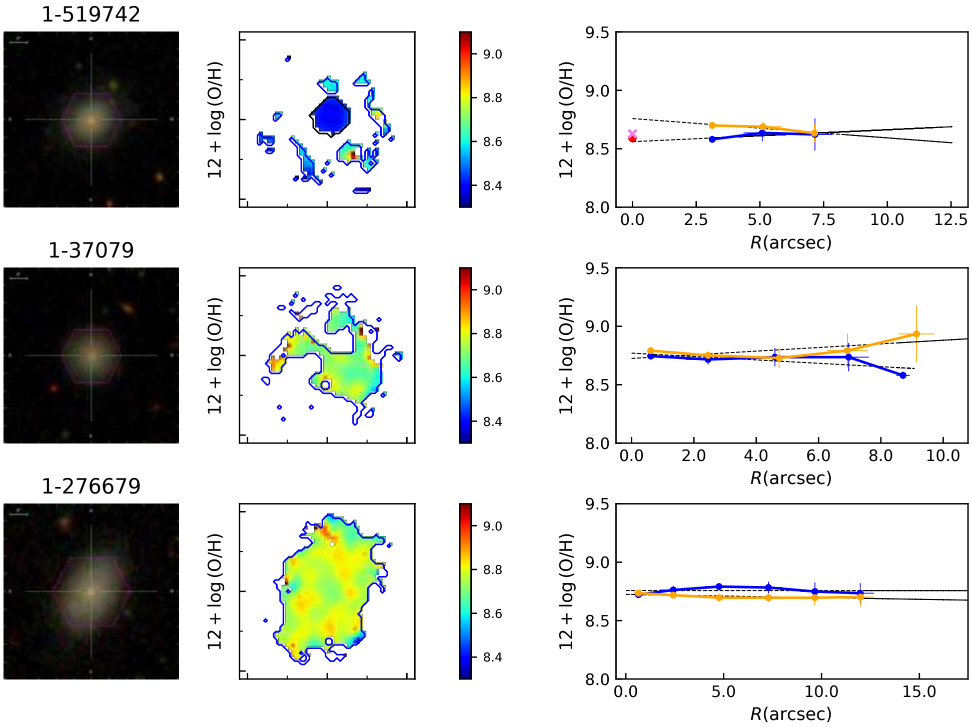


**Figure A28.** As Fig 3 but for the AGN host 1-519742.

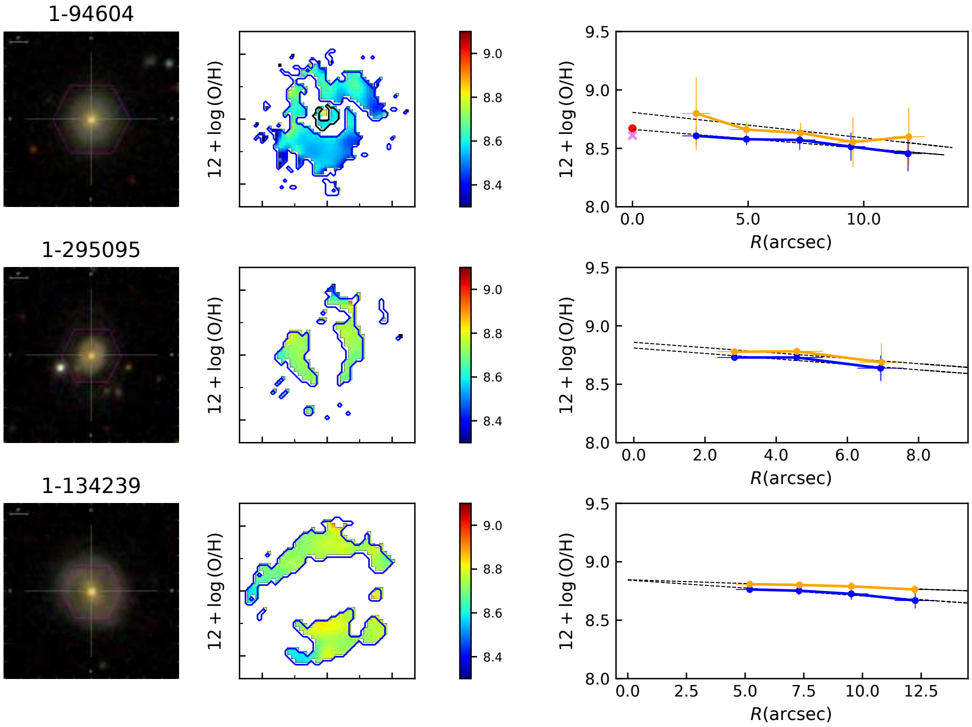


**Figure A29.** As Fig 3 but for the AGN host 1-94604.

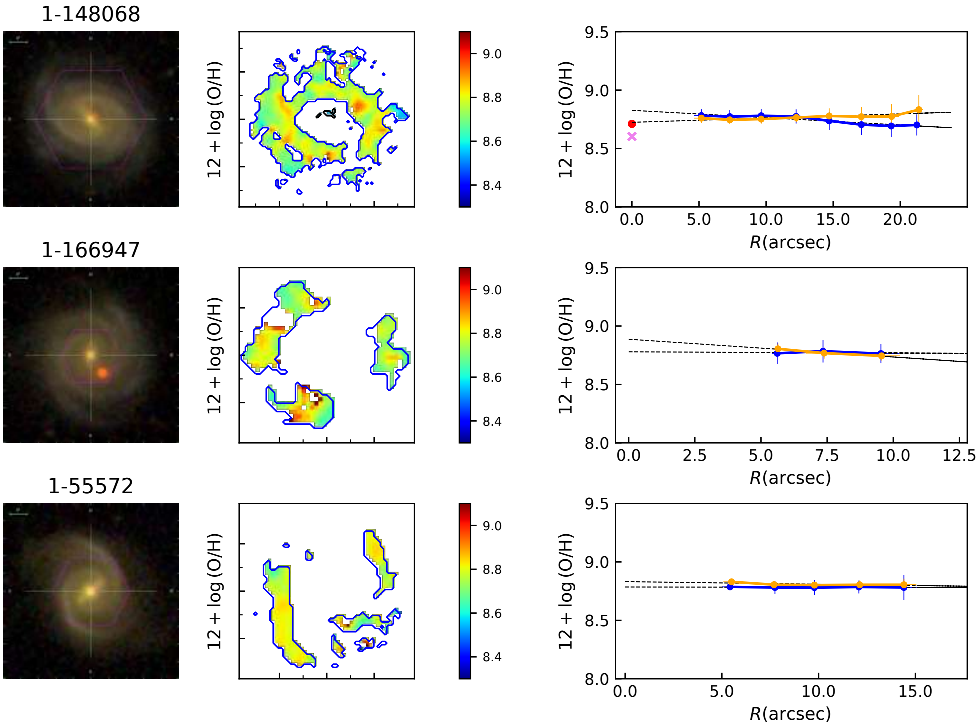


**Figure A30.** As Fig 3 but for the AGN host 1-148068.

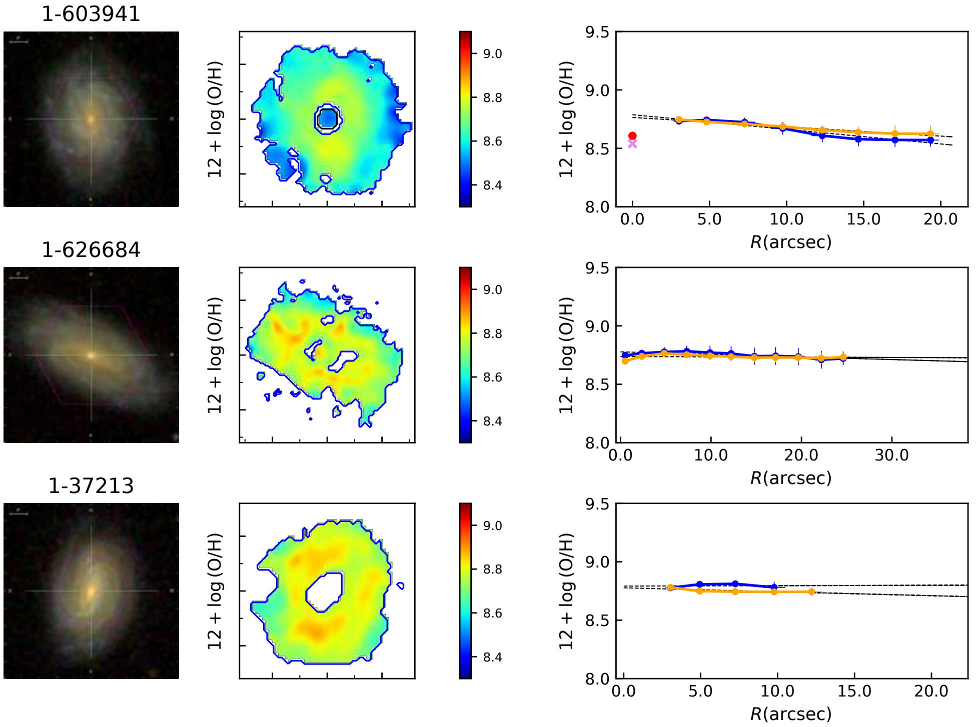


**Figure A31.** As Fig 3 but for the AGN host 1-603941.

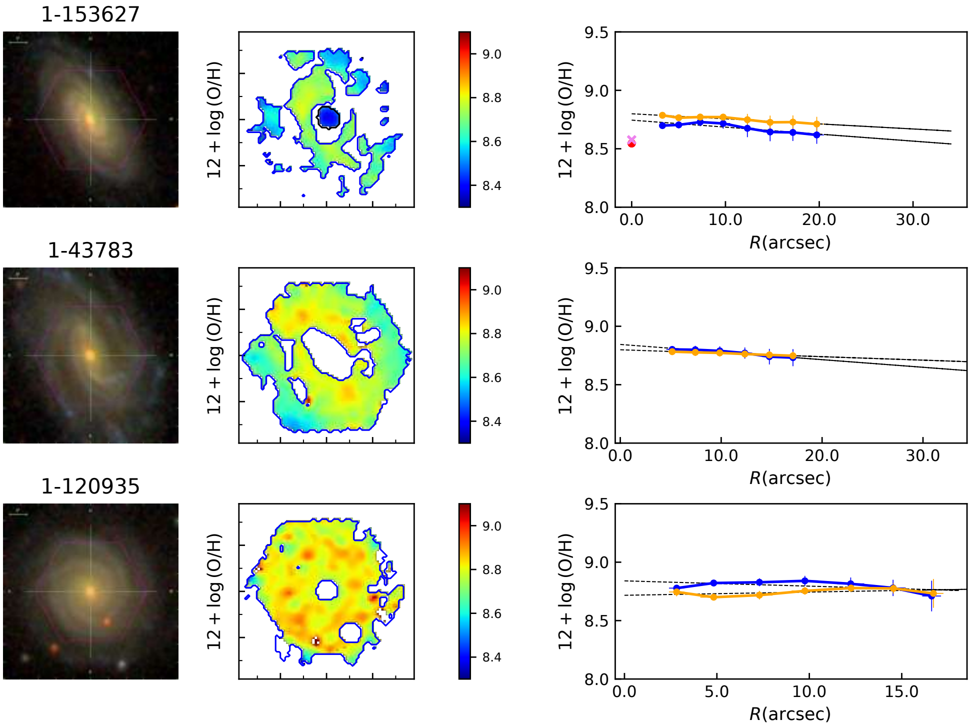


**Figure A32.** As Fig 3 but for the AGN host 1-153627.

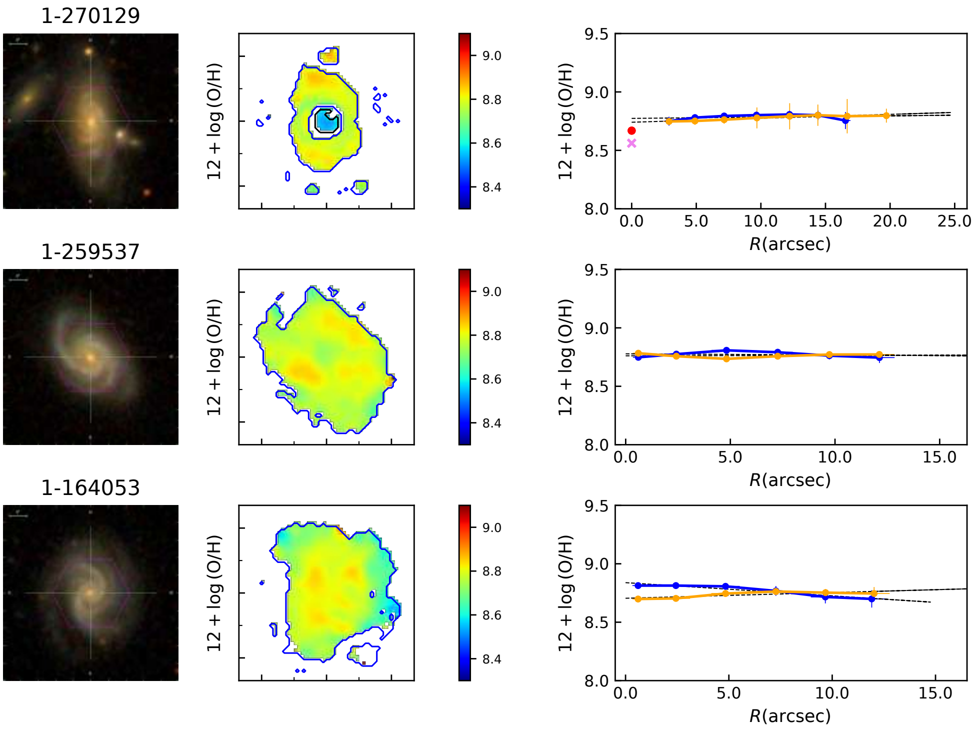


**Figure A33.** As Fig 3 but for the AGN host 1-270129.

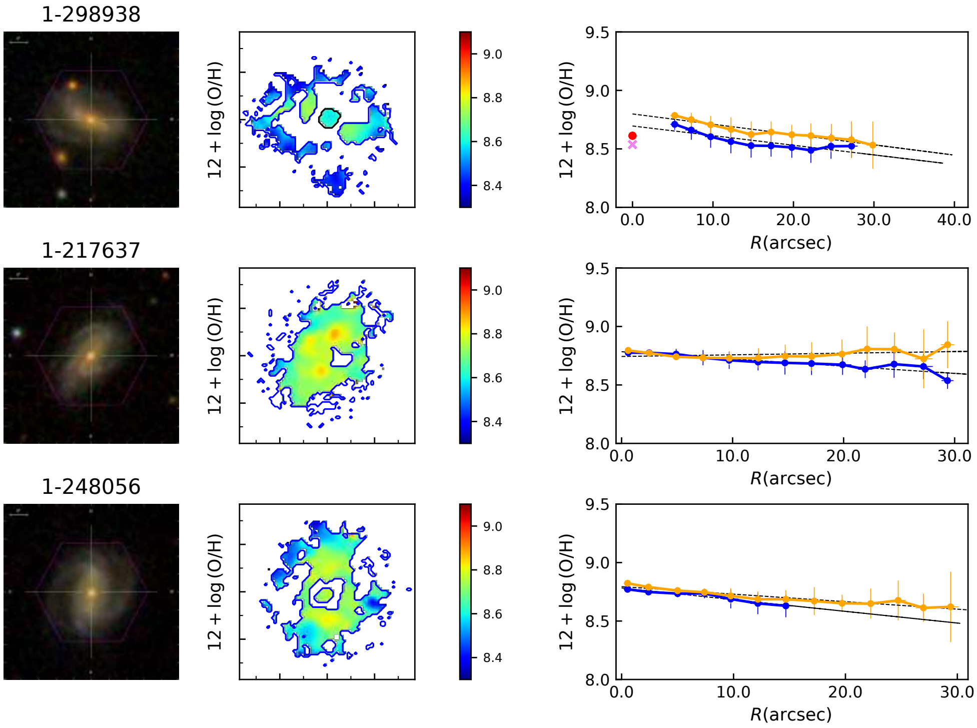


**Figure A34.** As Fig 3 but for the AGN host 1-298938.

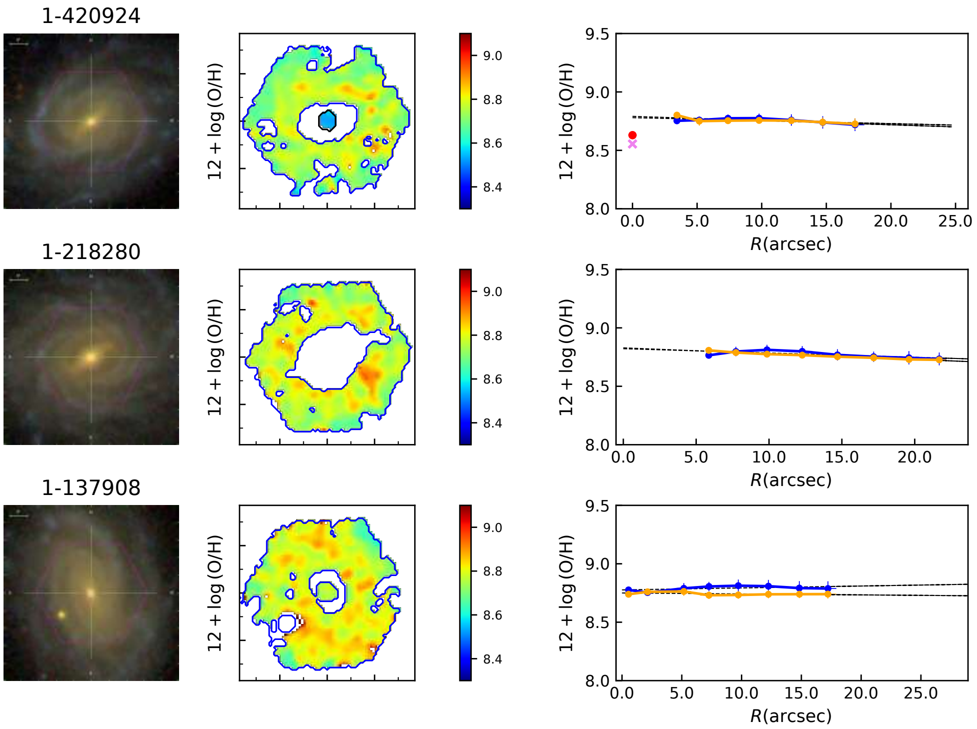


**Figure A35.** As Fig 3 but for the AGN host 1-420924.

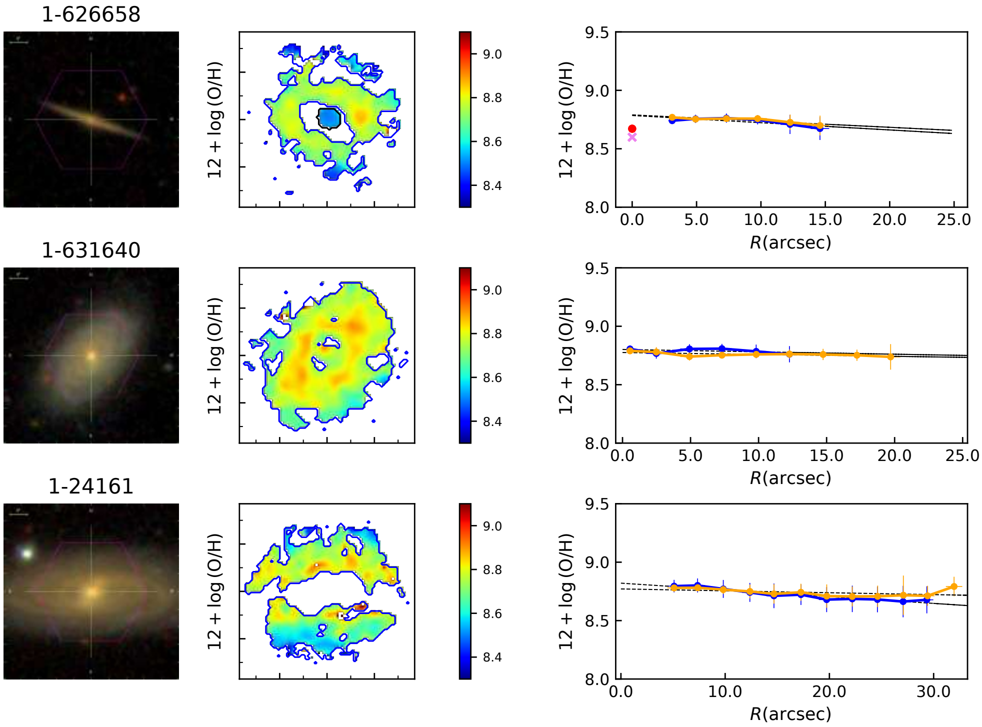


**Figure A36.** As Fig 3 but for the AGN host 1-626658.

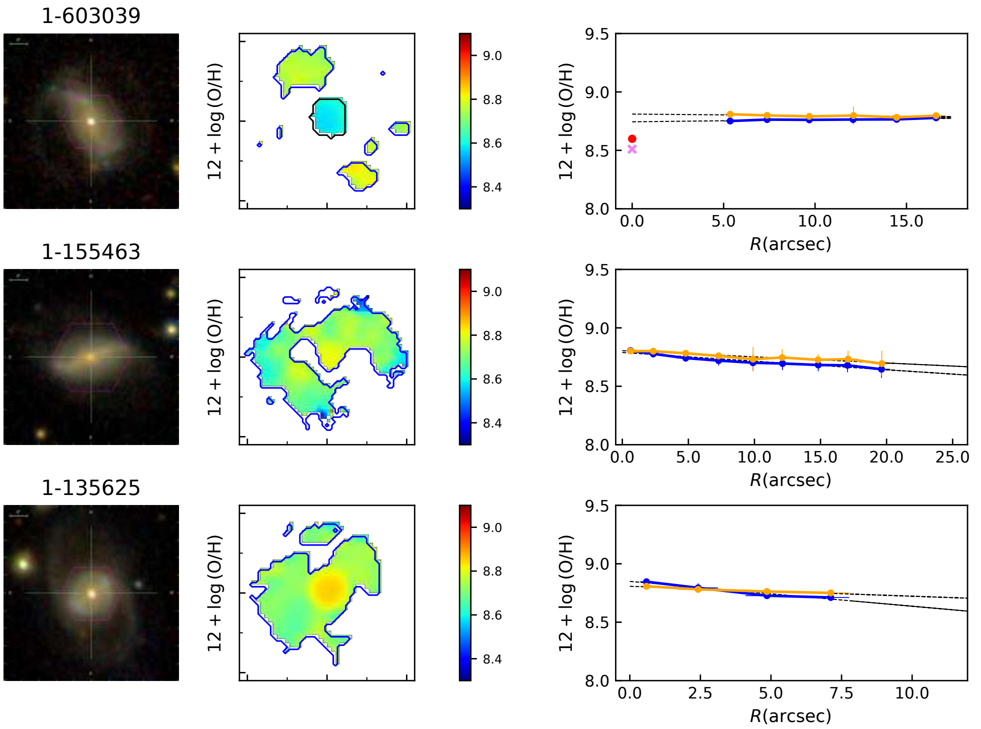


**Figure A37.** As Fig 3 but for the AGN host 1-603039.

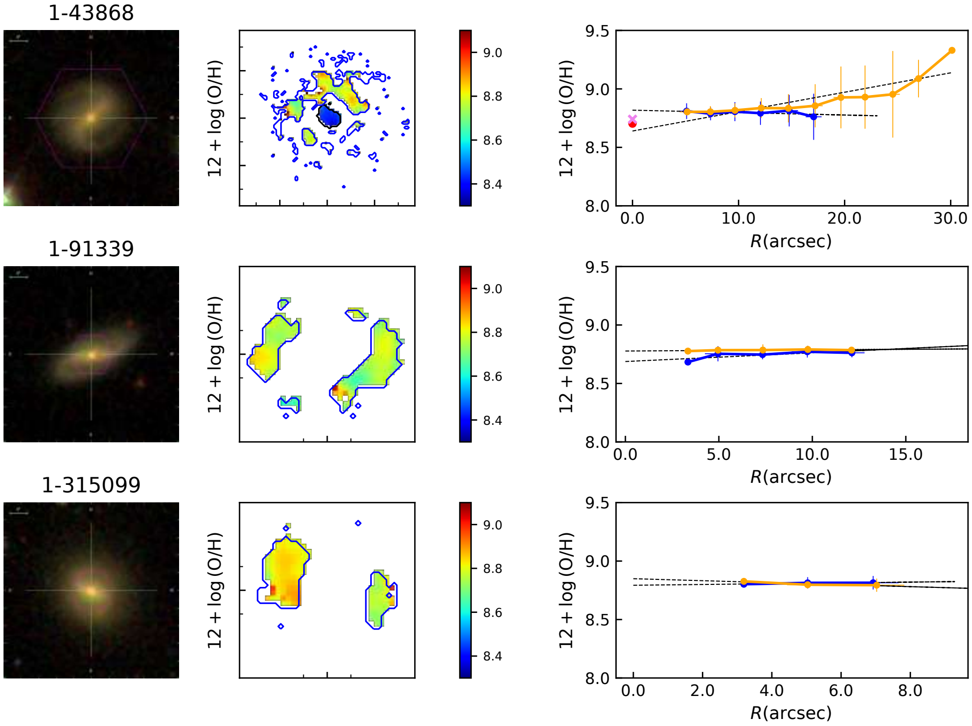


**Figure A38.** As Fig 3 but for the AGN host 1-43868.

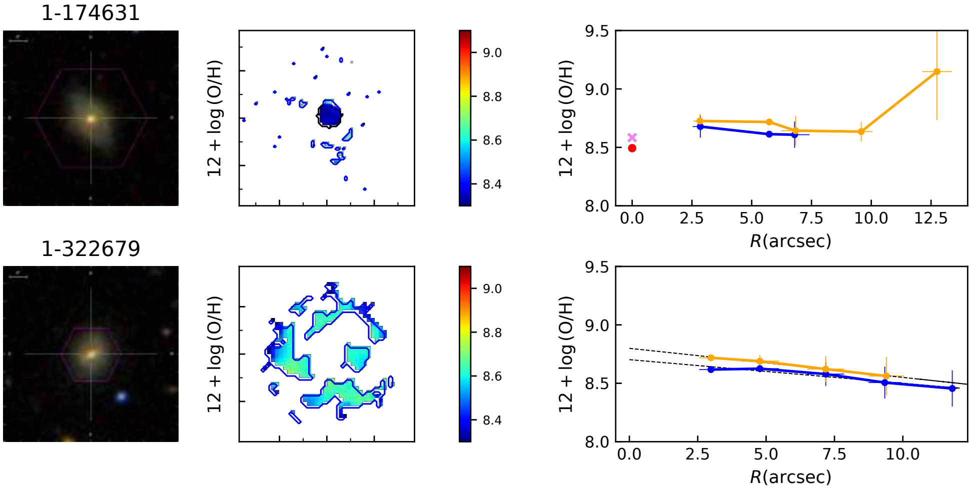


**Figure A39.** As Fig 3 but for the AGN host 1-174631.

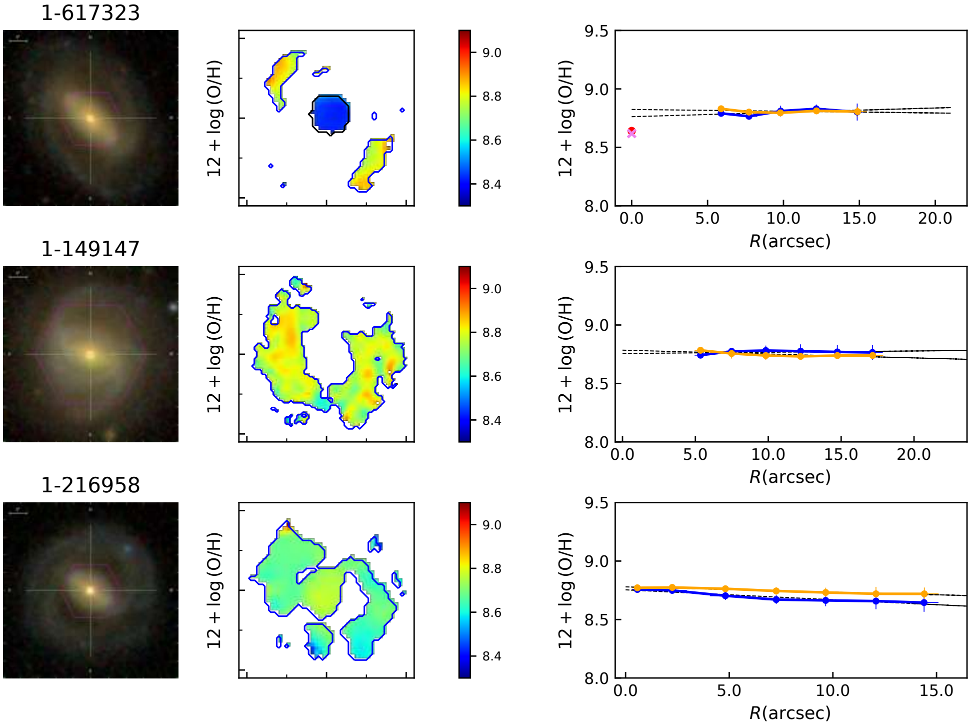


**Figure A40.** As Fig 3 but for the AGN host 1-617323.

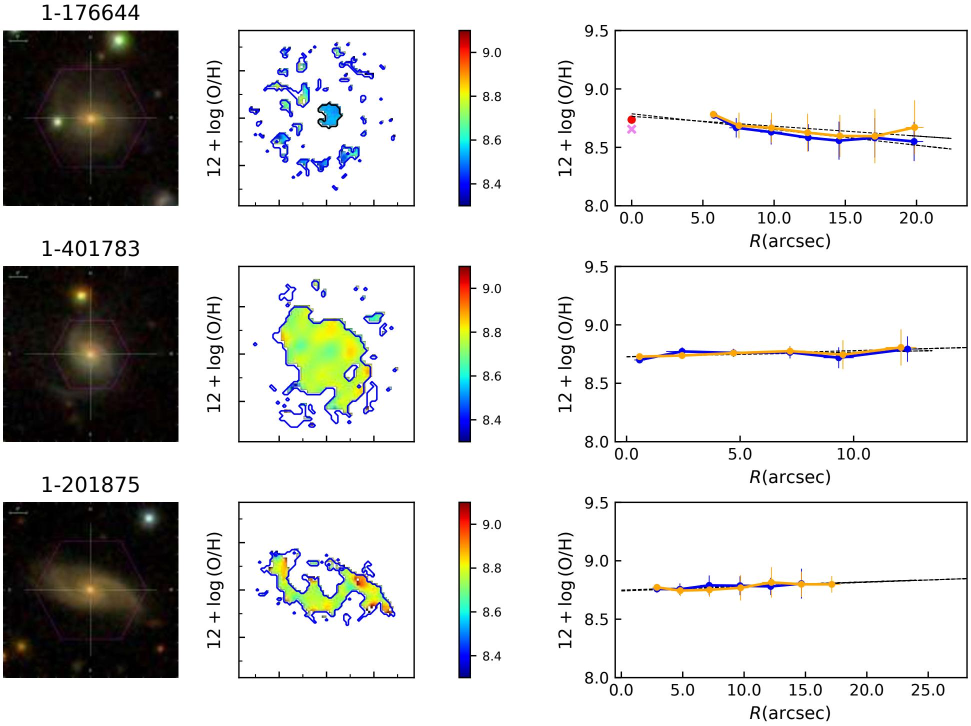


**Figure A41.** As Fig 3 but for the AGN host 1-176644.

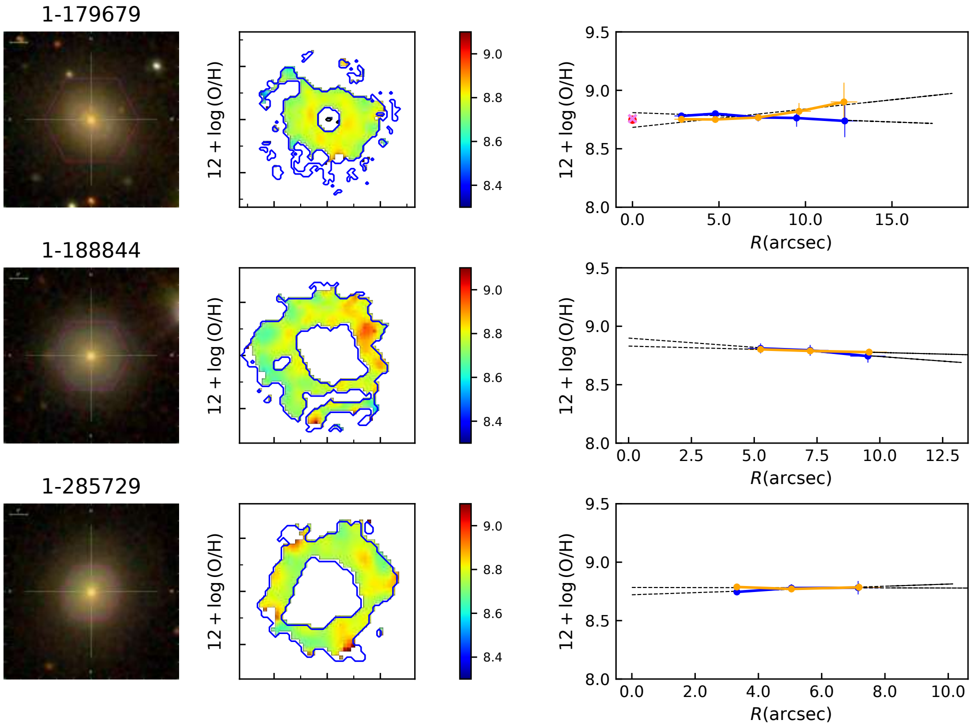


**Figure A42.** As Fig 3 but for the AGN host 1-179679.

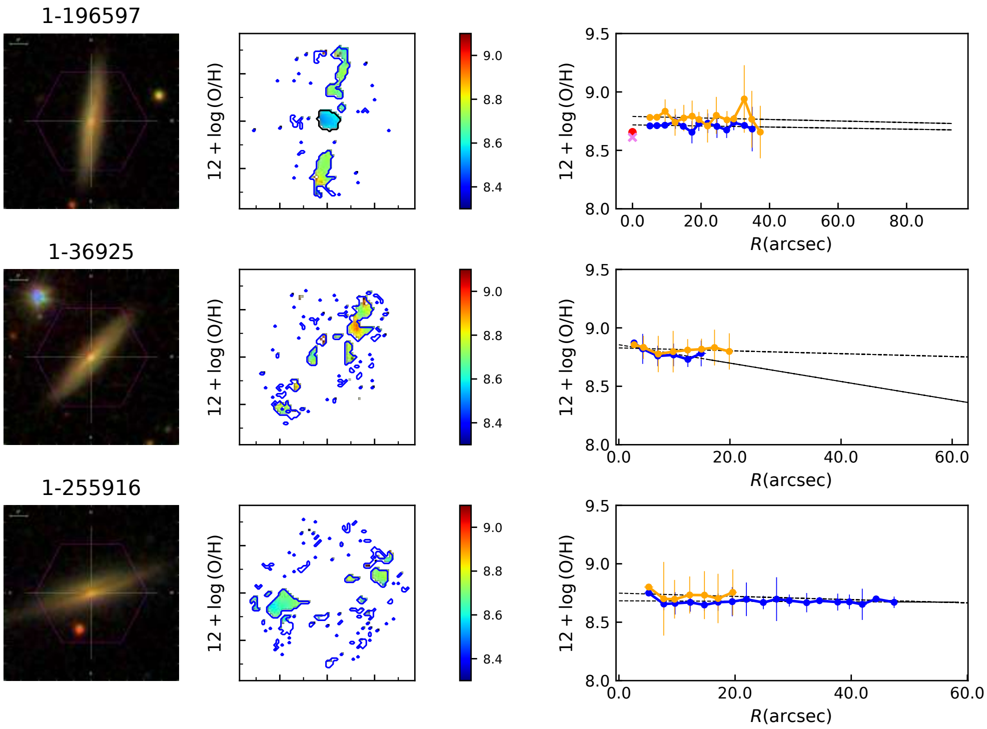


**Figure A43.** As Fig 3 but for the AGN host 1-196597.

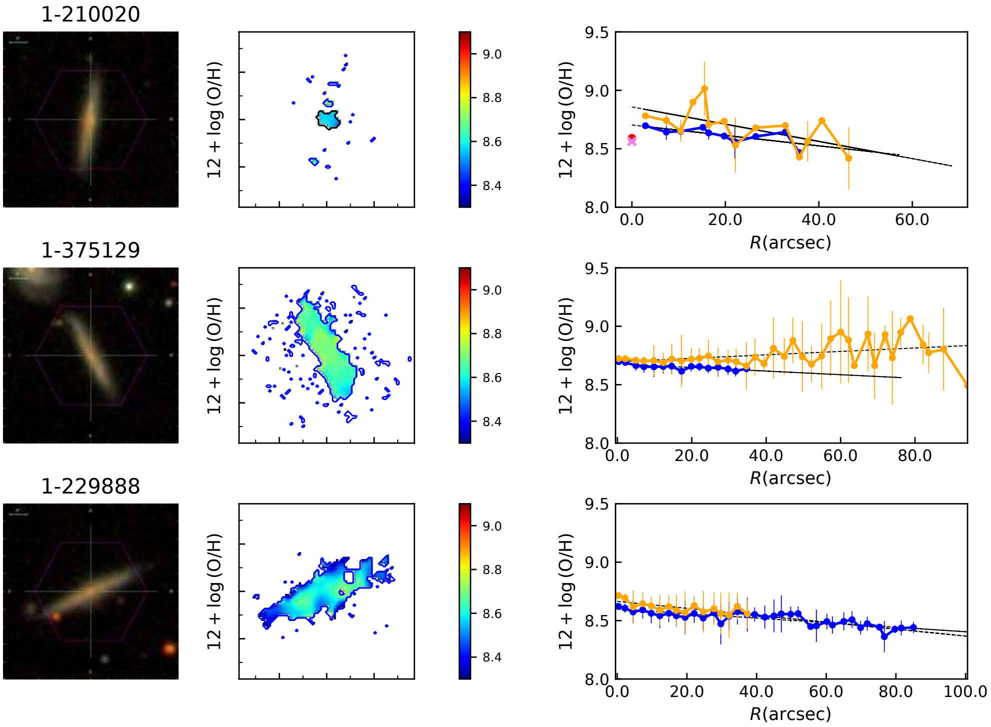


**Figure A44.** As Fig 3 but for the AGN host 1-210020.

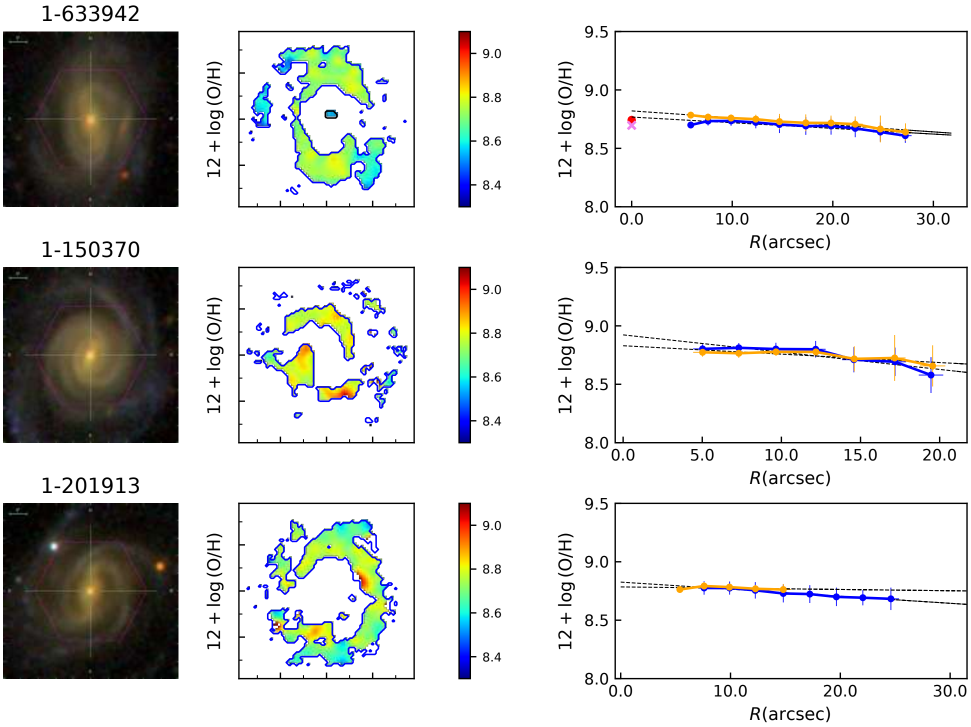


**Figure A45.** As Fig 3 but for the AGN host 1-633942.

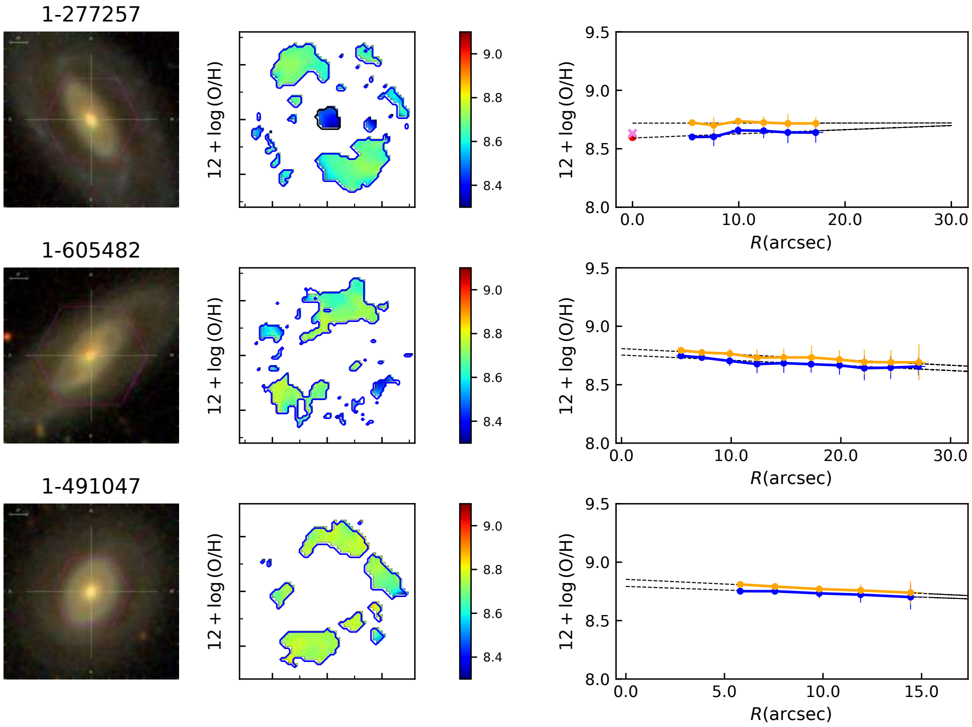


**Figure A46.** As Fig 3 but for the AGN host 1-277257.

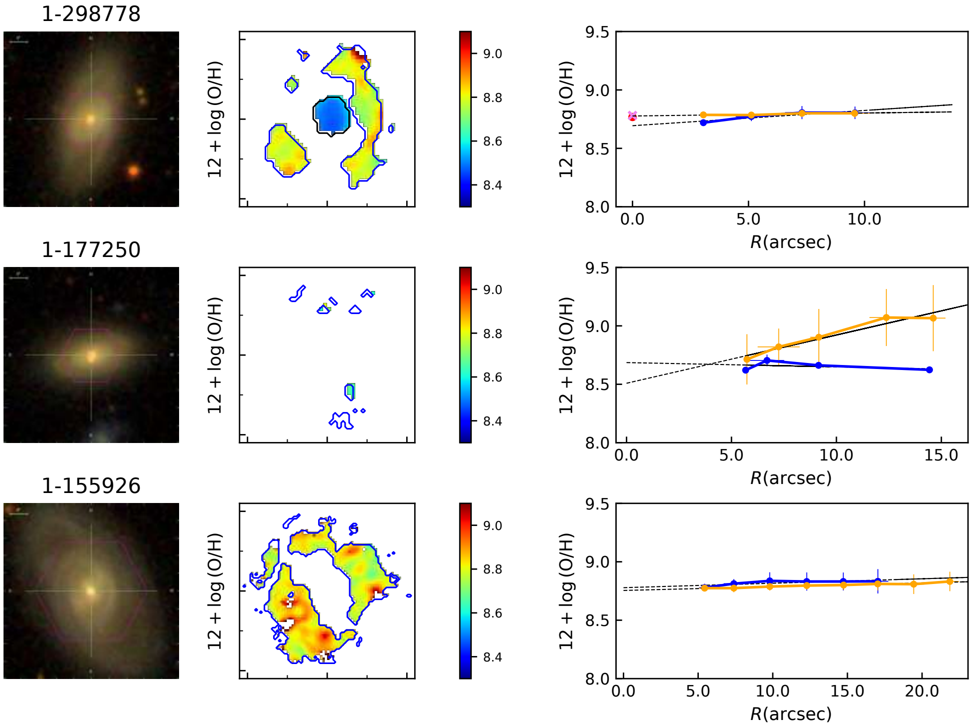


**Figure A47.** As Fig 3 but for the AGN host 1-298778.

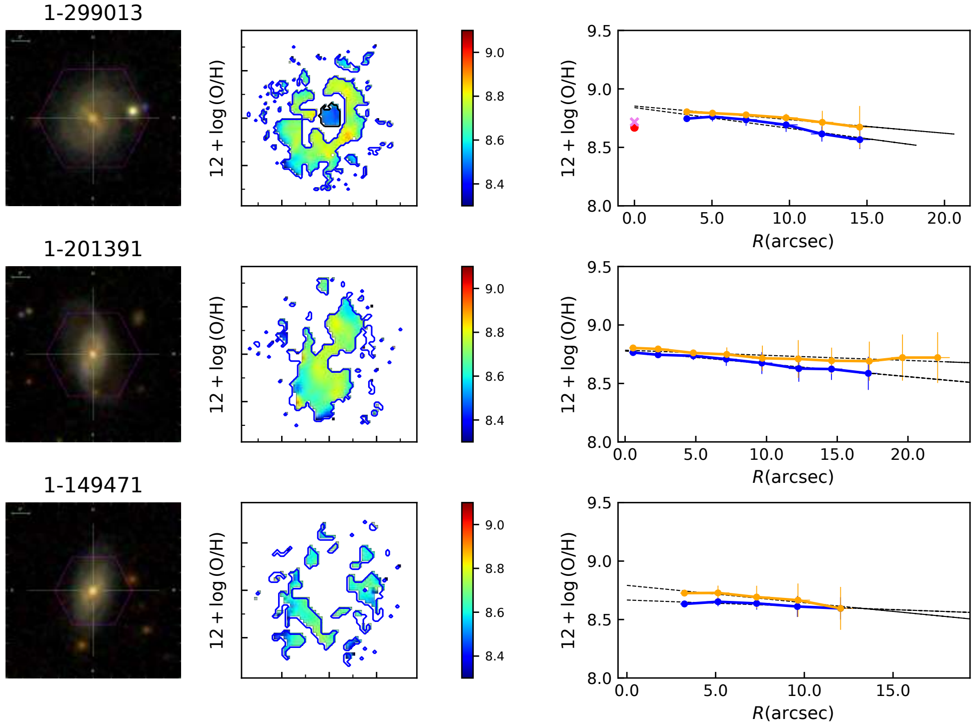


**Figure A48.** As Fig 3 but for the AGN host 1-299013.

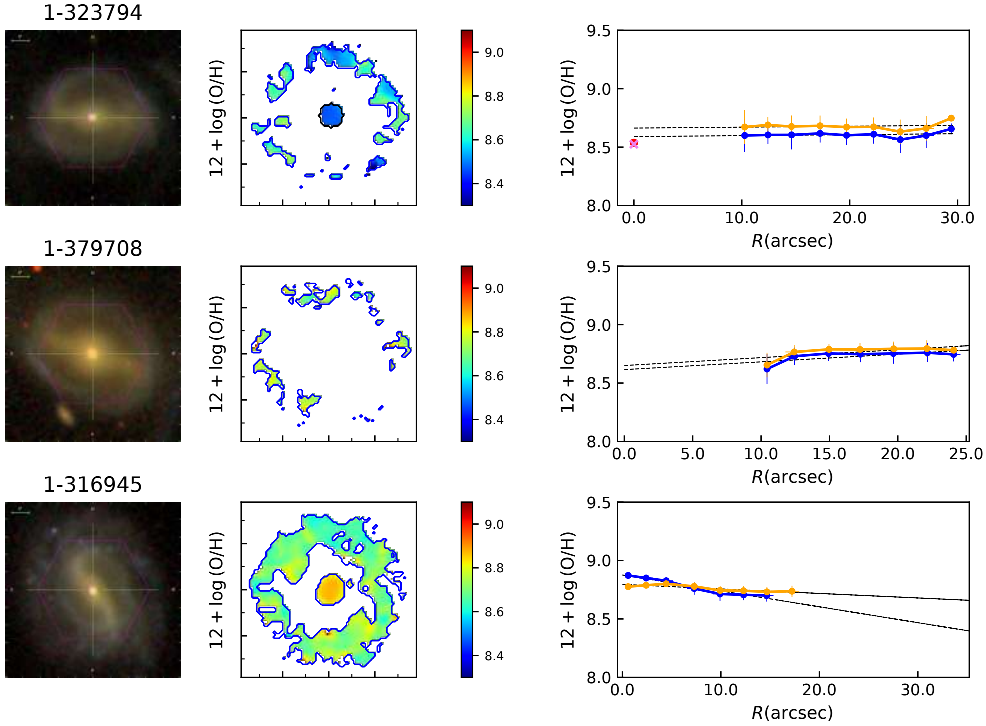


**Figure A49.** As Fig 3 but for the AGN host 1-323794.

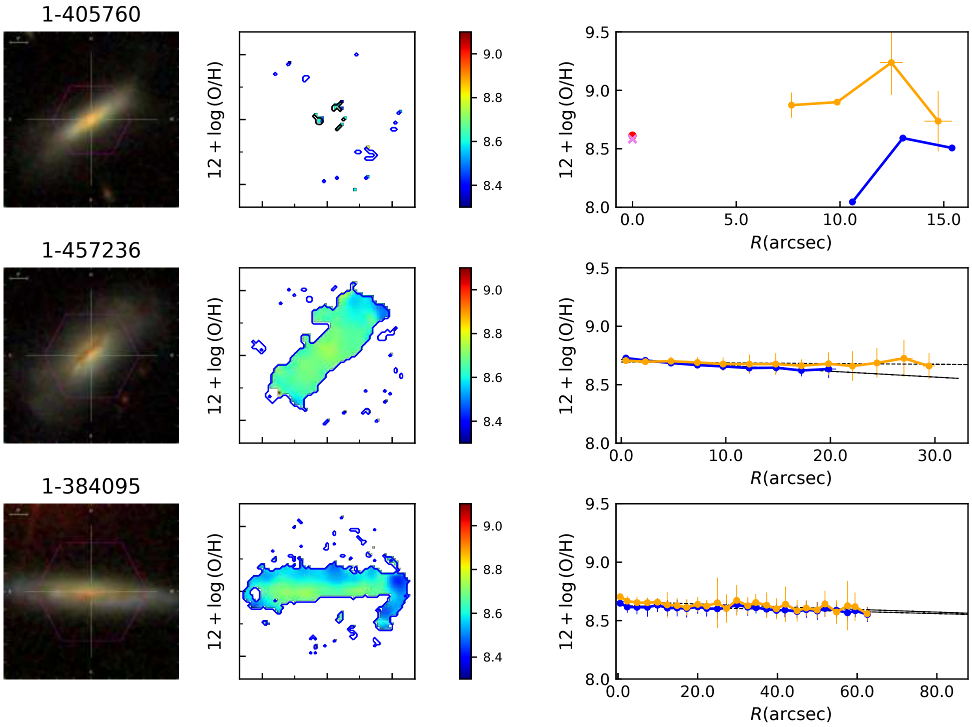


**Figure A50.** As Fig 3 but for the AGN host 1-405760.

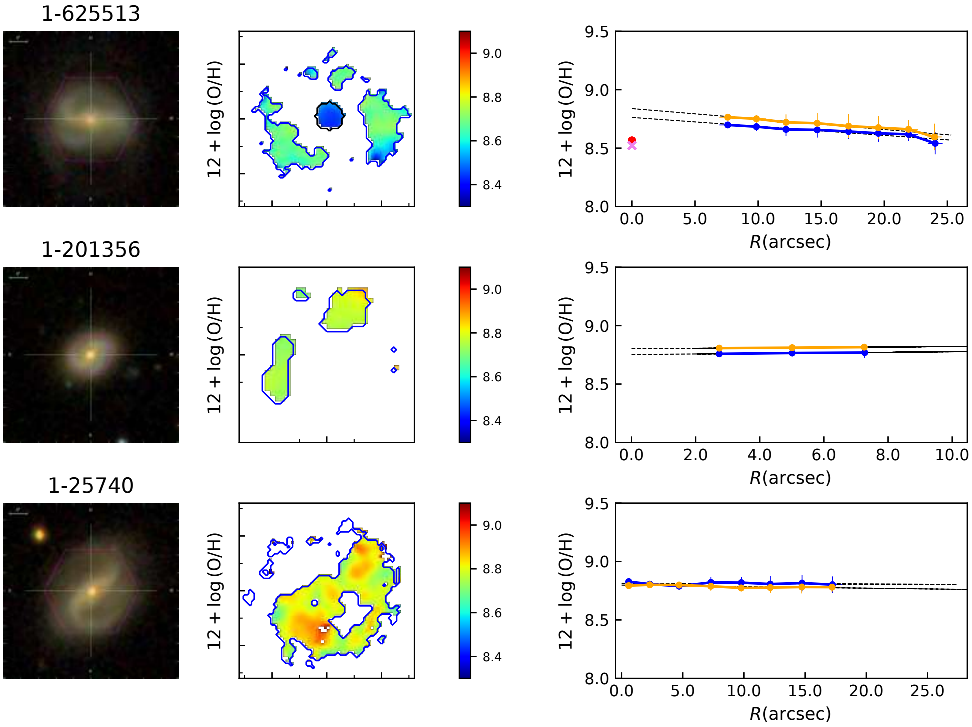


**Figure A51.** As Fig 3 but for the AGN host 1-625513.

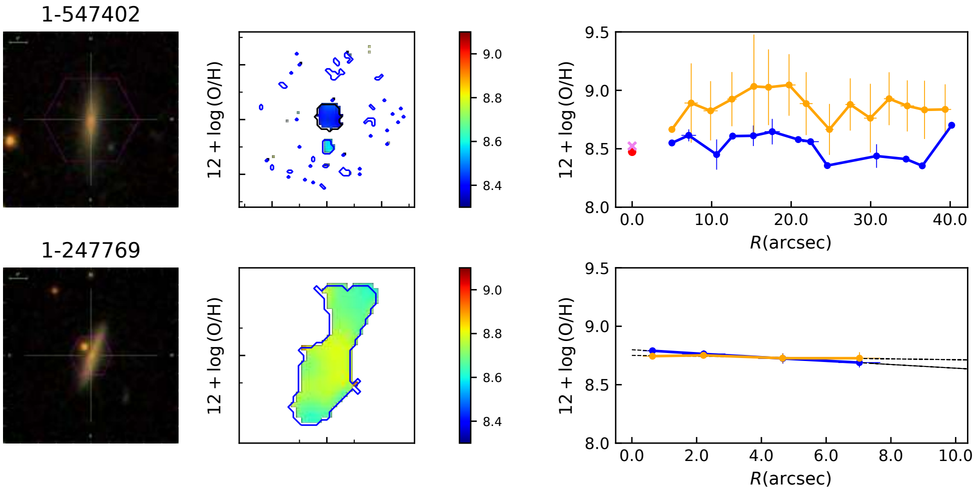


**Figure A52.** As Fig 3 but for the AGN host 1-547402.

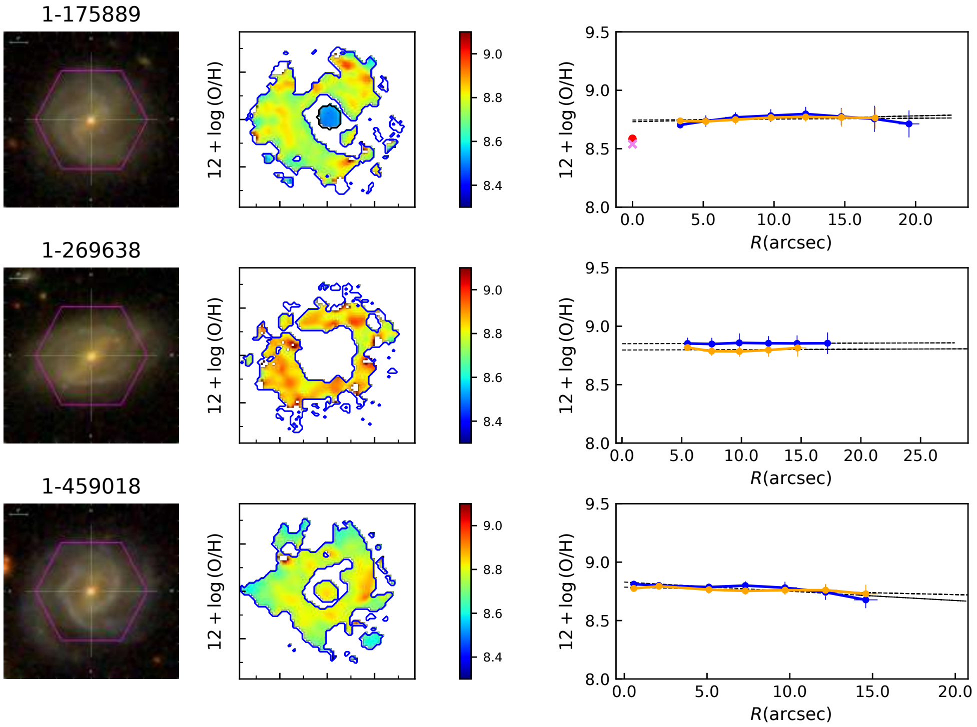


**Figure A53.** As Fig 3 but for the AGN host 1-175889.

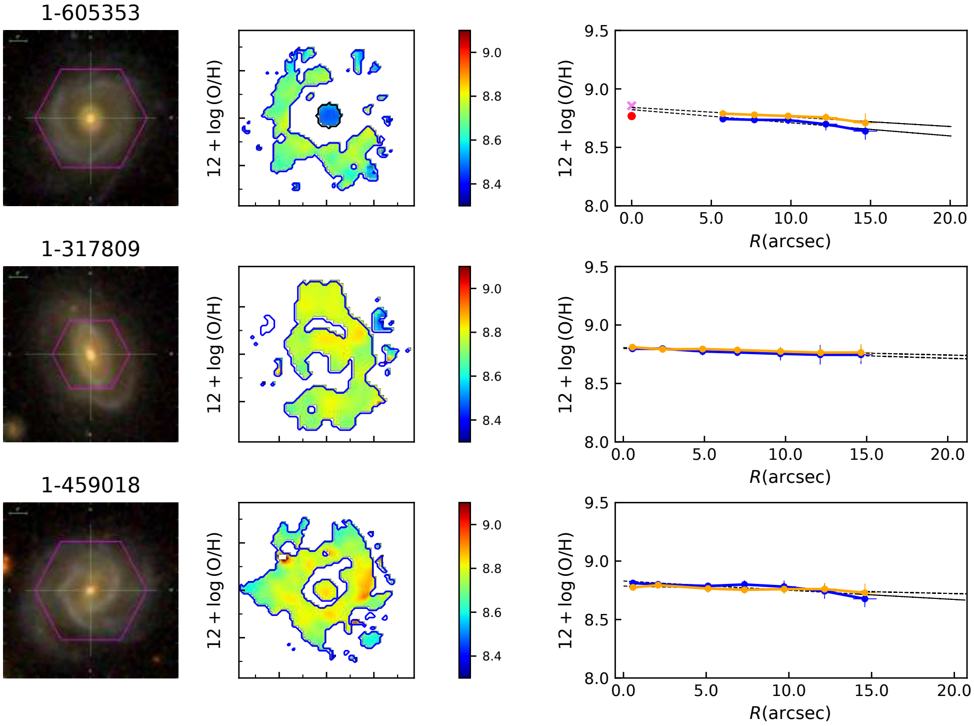


**Figure A54.** As Fig 3 but for the AGN host 1-605353.

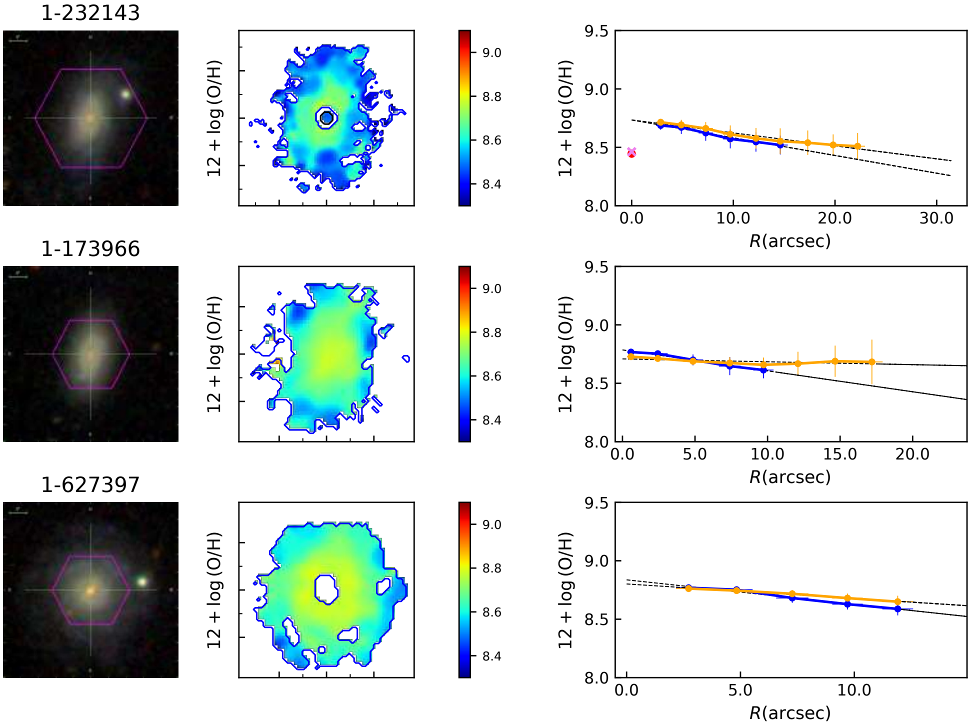


**Figure A55.** As Fig 3 but for the AGN host 1-232143.

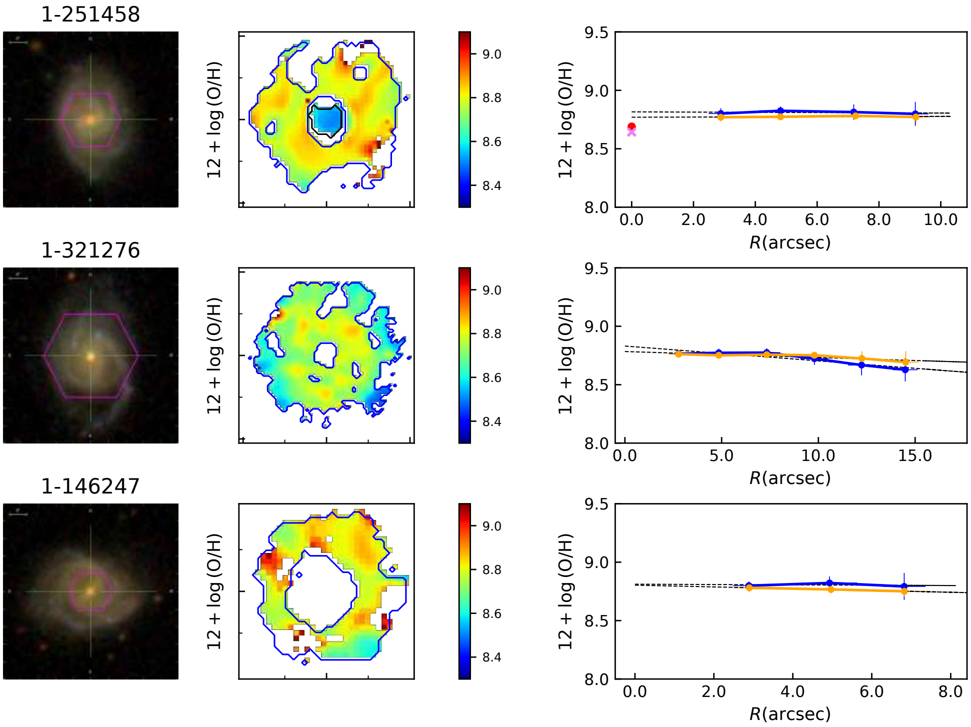


**Figure A56.** As Fig 3 but for the AGN host 1-251458.

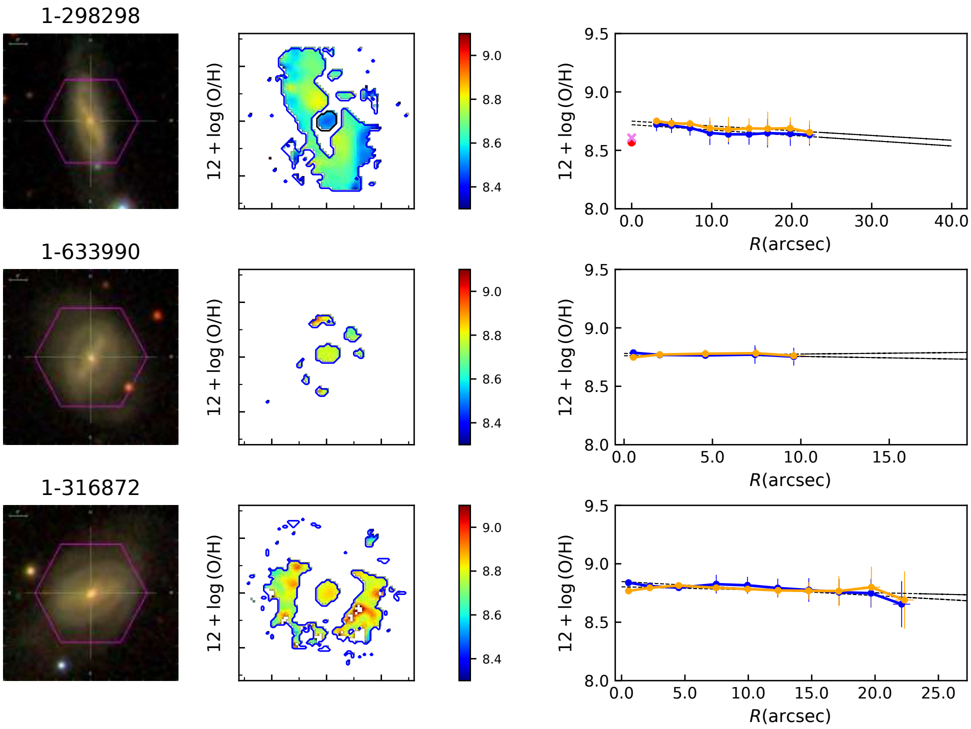


**Figure A57.** As Fig 3 but for the AGN host 1-298298.

This paper has been typeset from a TeX/LaTeX file prepared by the author.

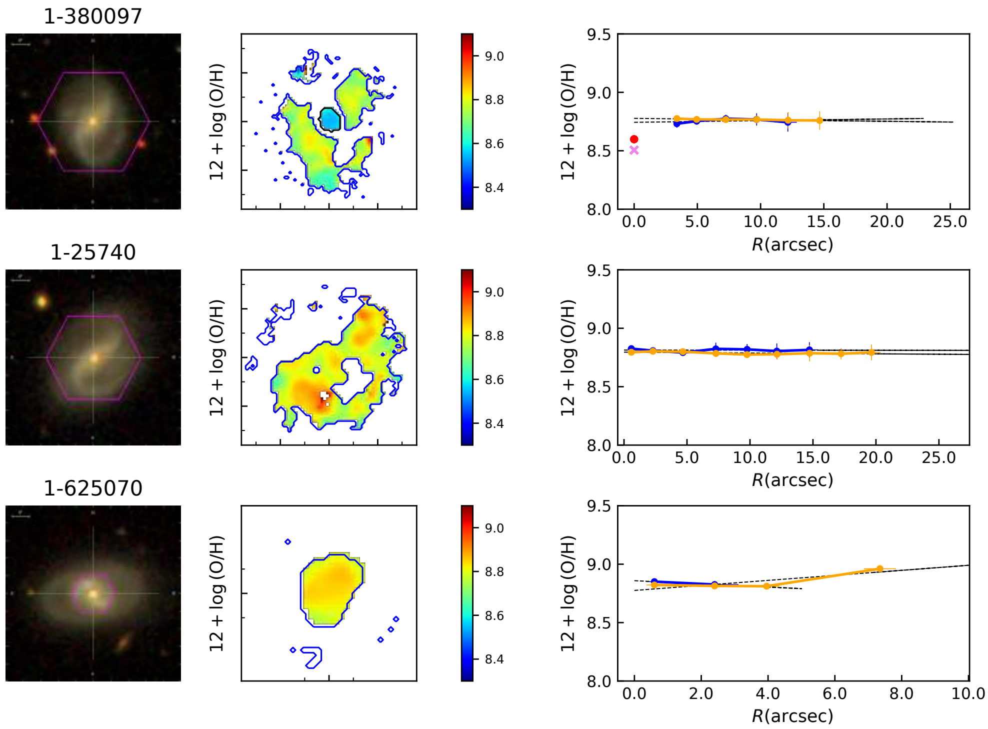


**Figure A58.** As Fig 3 but for the AGN host 1-380097.

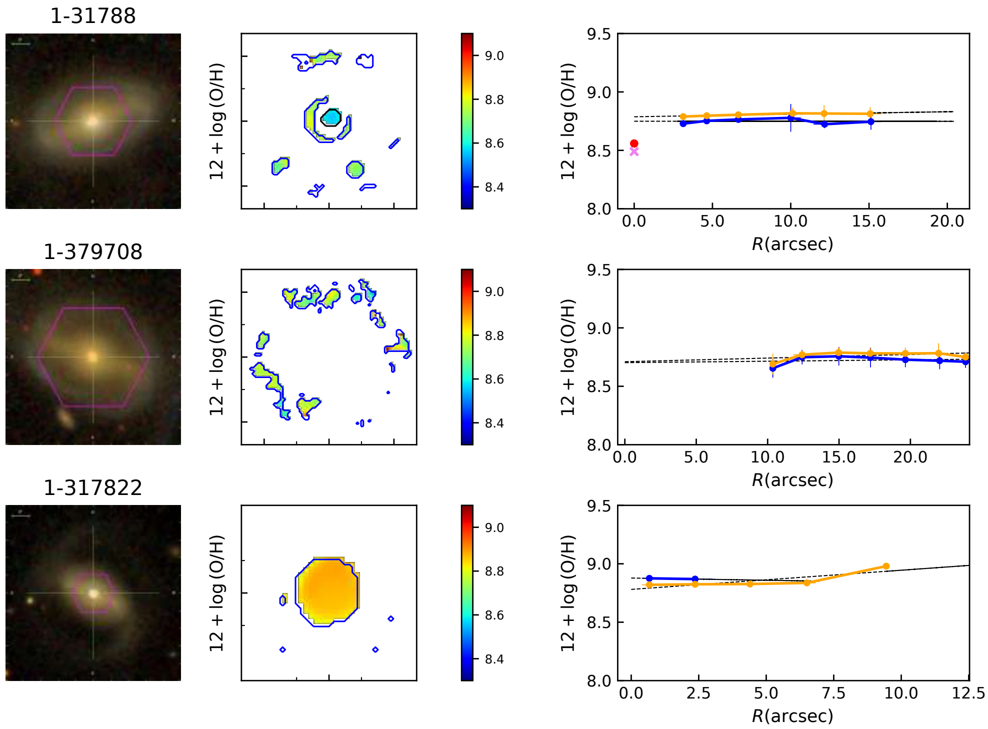


**Figure A59.** As Fig 3 but for the AGN host 1-31788.

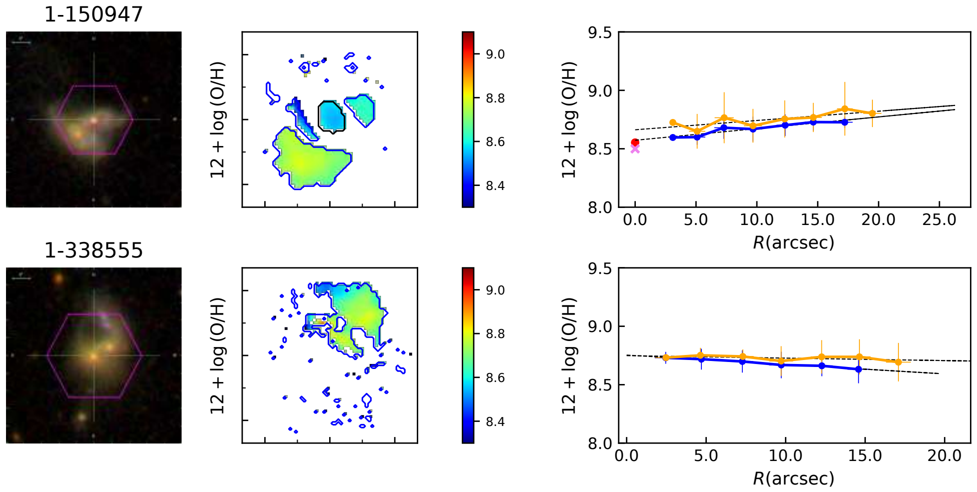


**Figure A60.** As Fig 3 but for the AGN host 1-150947

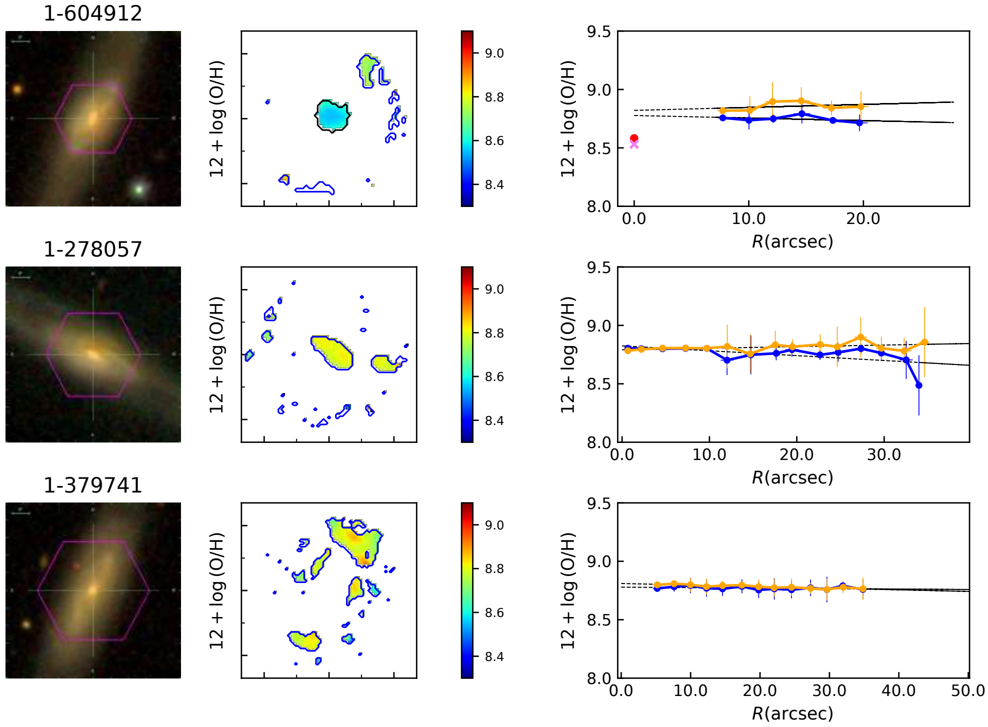


**Figure A61.** As Fig 3 but for the AGN host 1-604912.

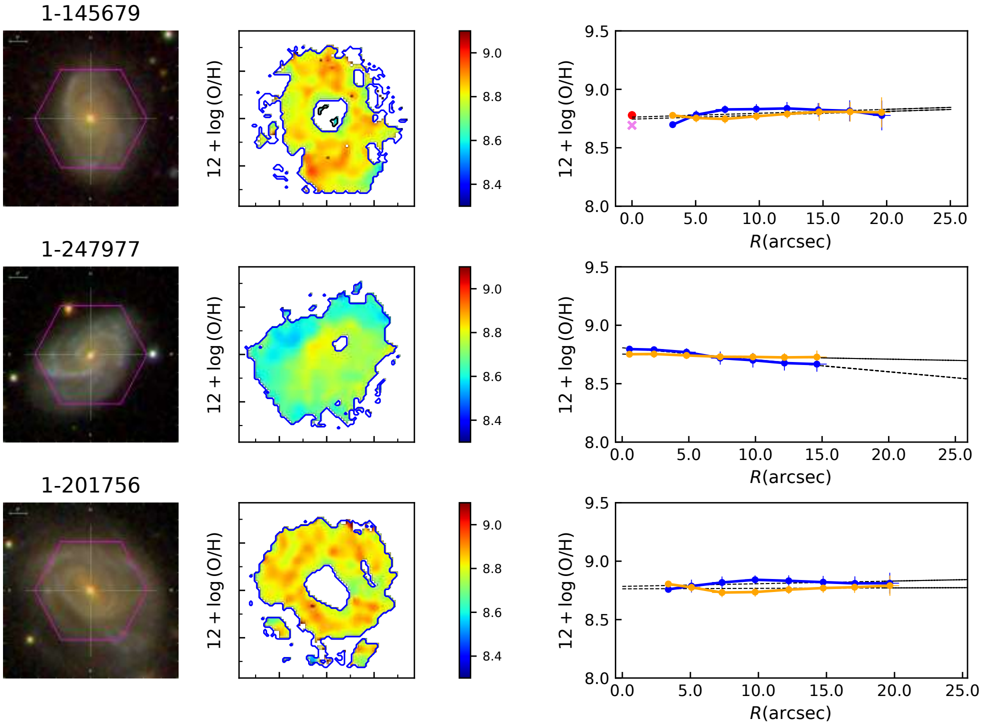


**Figure A62.** As Fig 3 but for the AGN host 1-145679

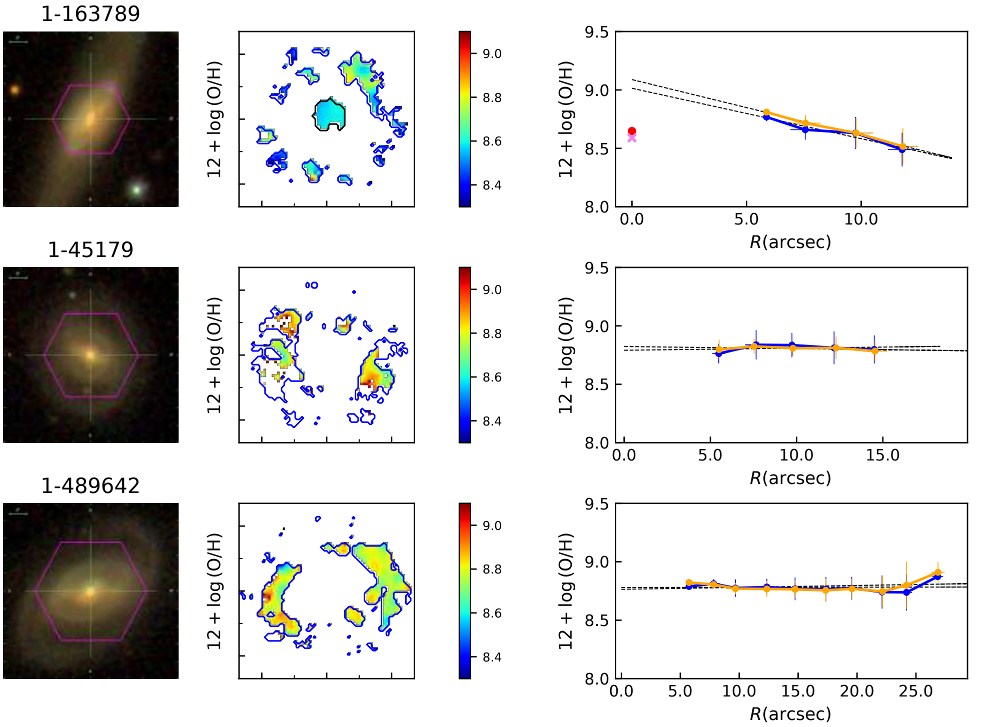


**Figure A63.** As Fig 3 but for the AGN host 1-163789.

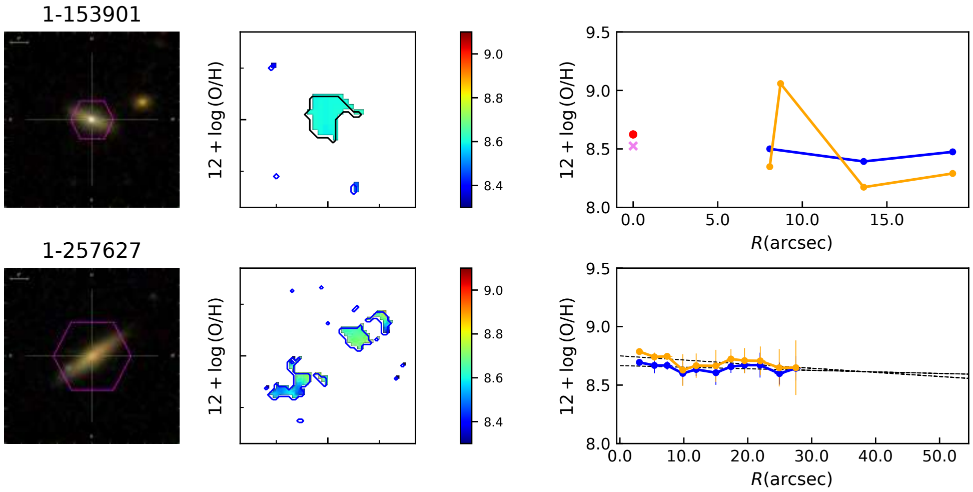


**Figure A64.** As Fig 3 but for the AGN host 1-153901.

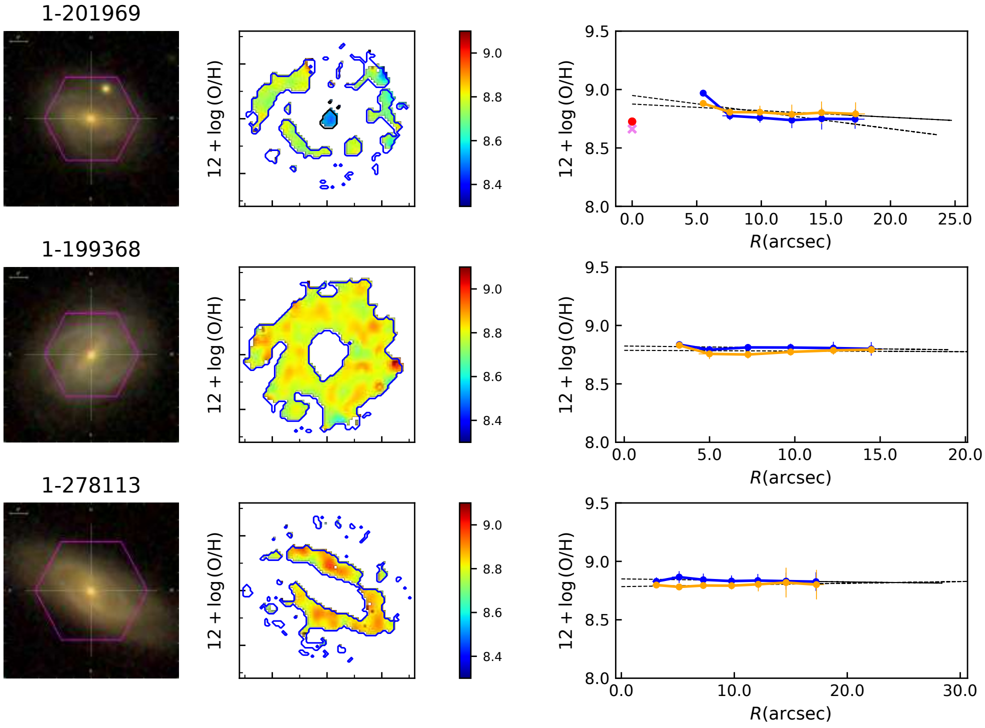


**Figure A65.** As Fig 3 but for the AGN host 1-201969.

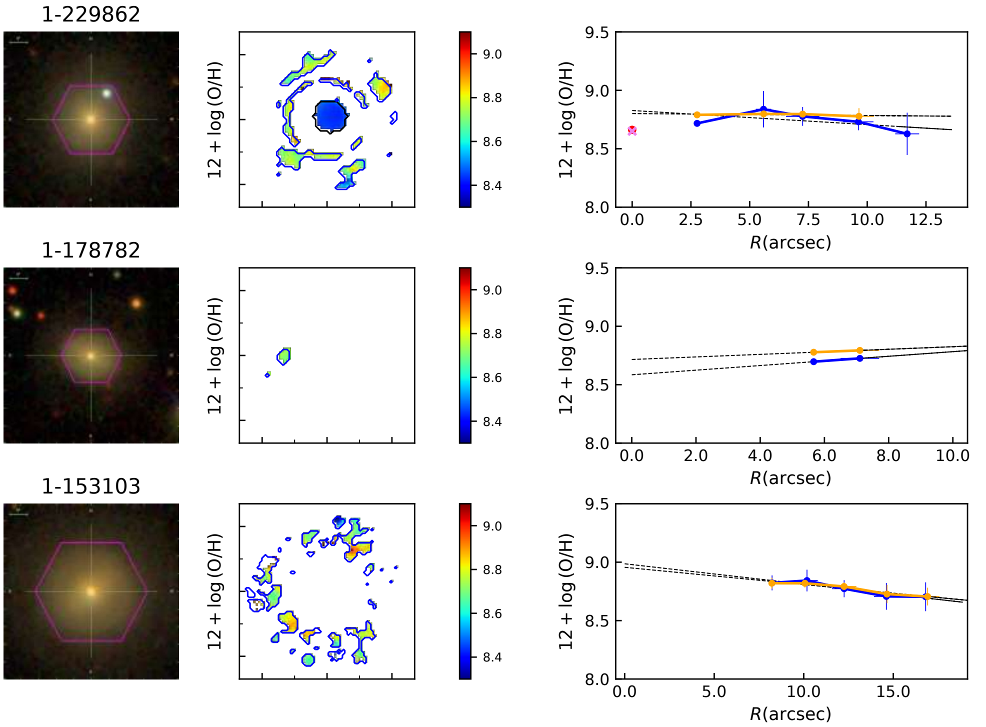


**Figure A66.** As Fig 3 but for the AGN host 1-229862.

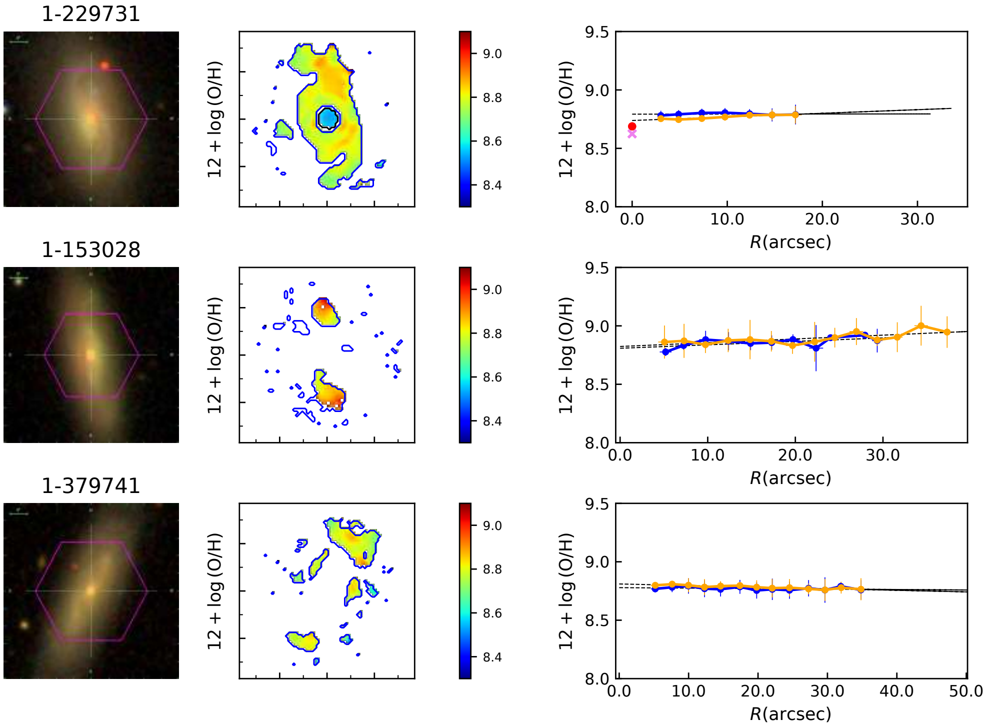


**Figure A67.** As Fig 3 but for the AGN host 1-229731.

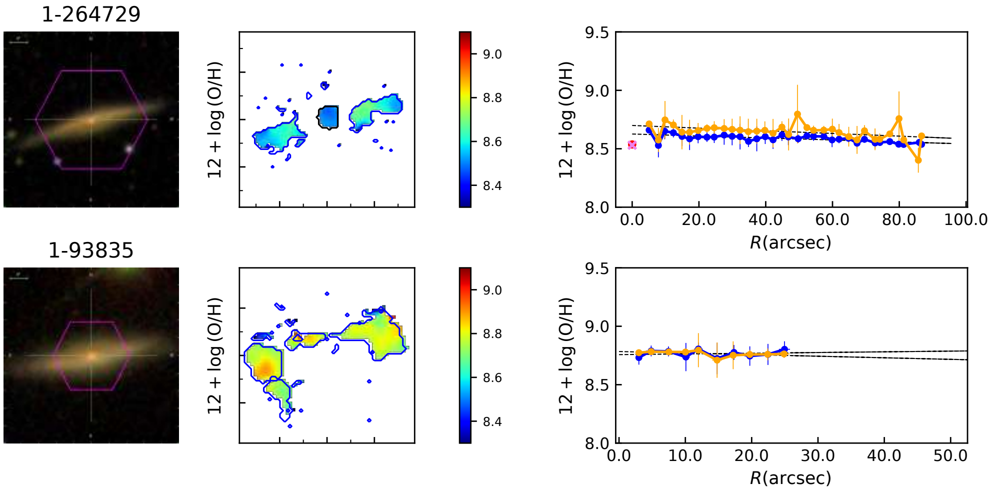


**Figure A68.** As Fig 3 but for the AGN host 1-264729.

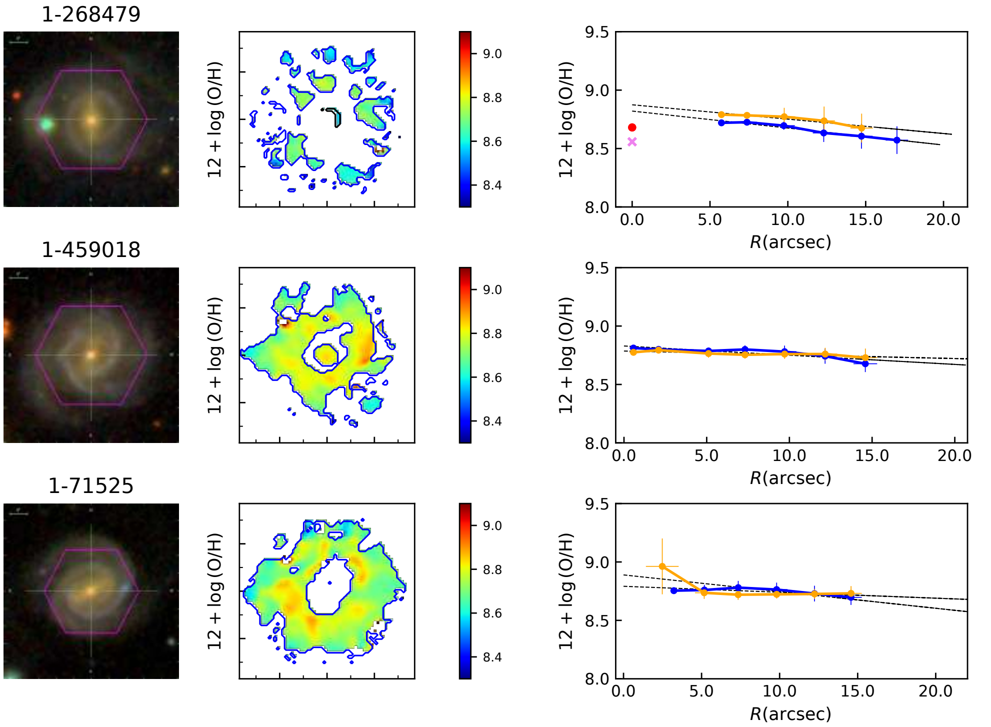


**Figure A69.** As Fig 3 but for the AGN host 1-268479.

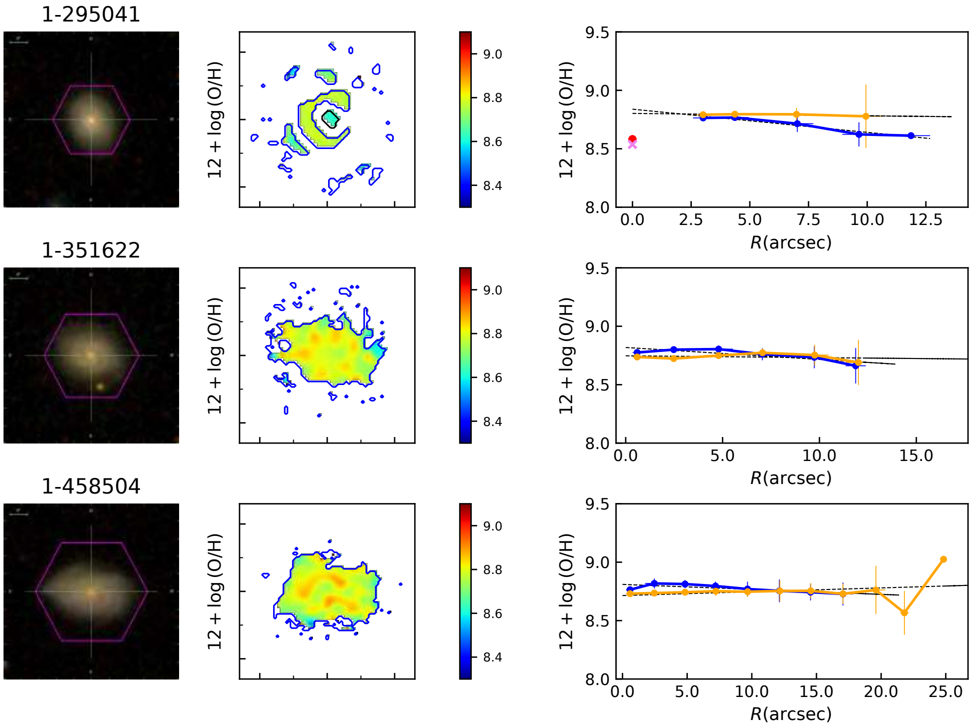


**Figure A70.** As Fig 3 but for the AGN host 1-295041.

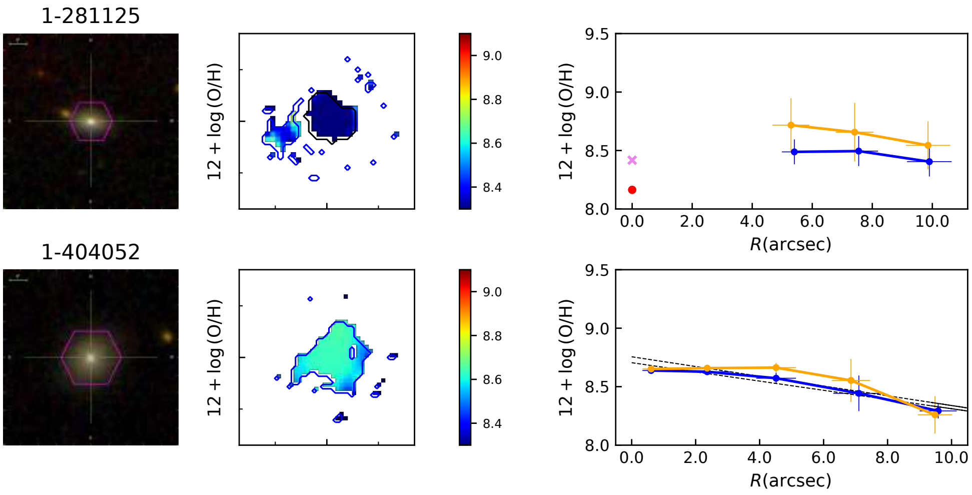


**Figure A71.** As Fig 3 but for the AGN host 1-281125.

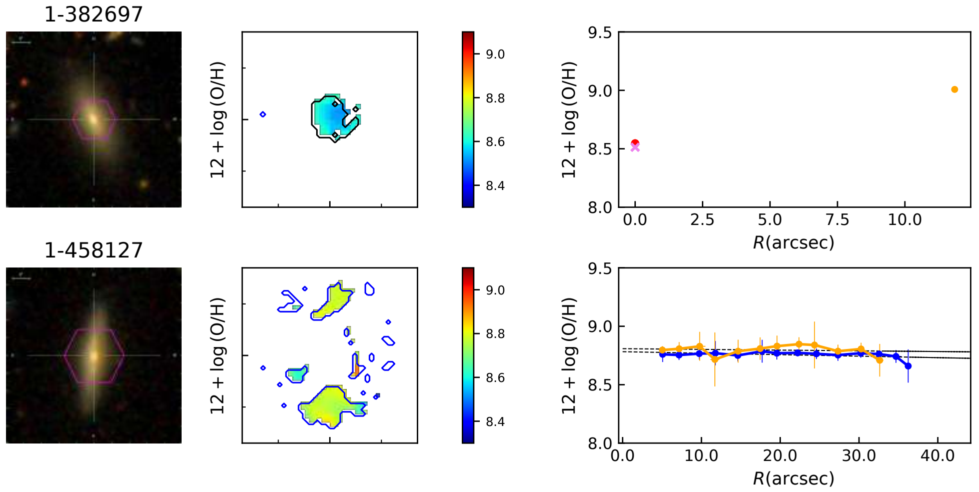


**Figure A72.** As Fig 3 but for the AGN host 1-382697.

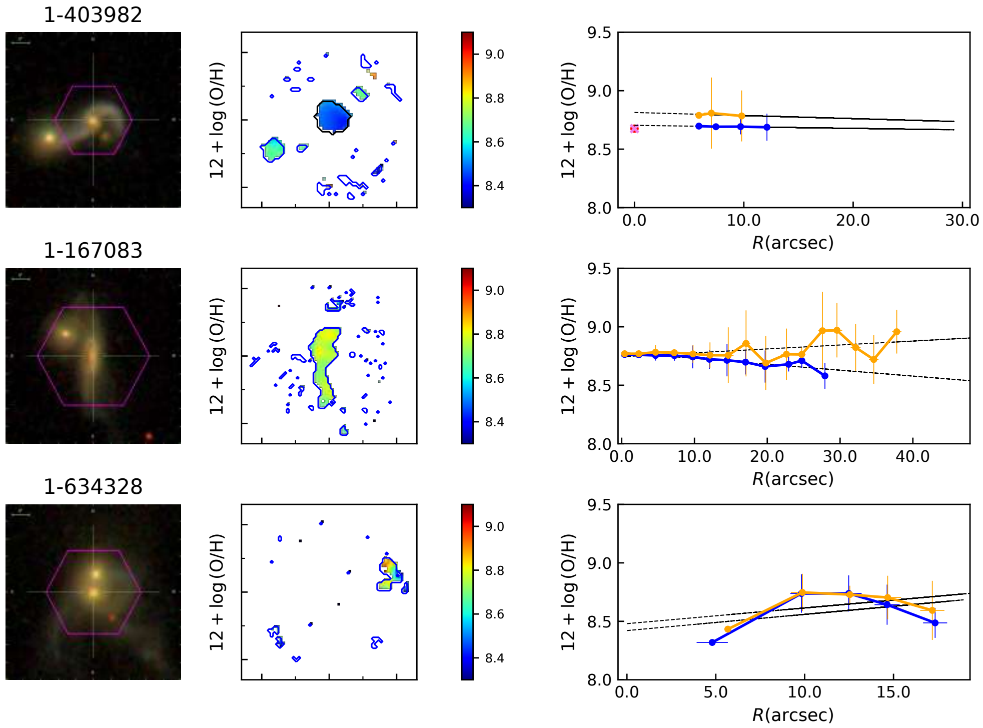


**Figure A73.** As Fig 3 but for the AGN host 1-403982.

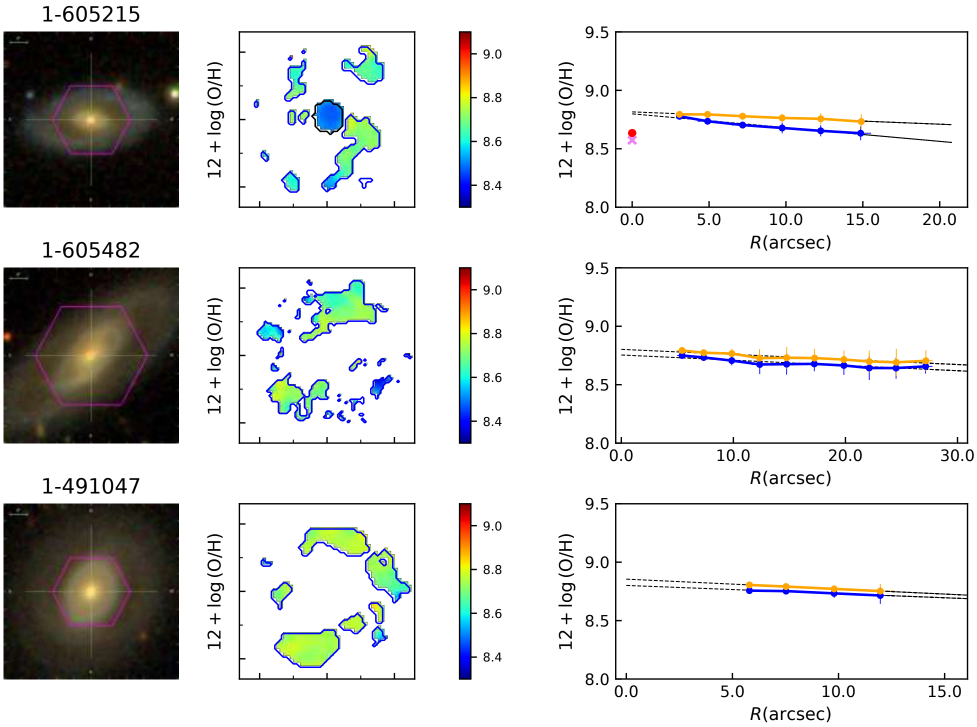


**Figure A74.** As Fig 3 but for the AGN host 1-605215.

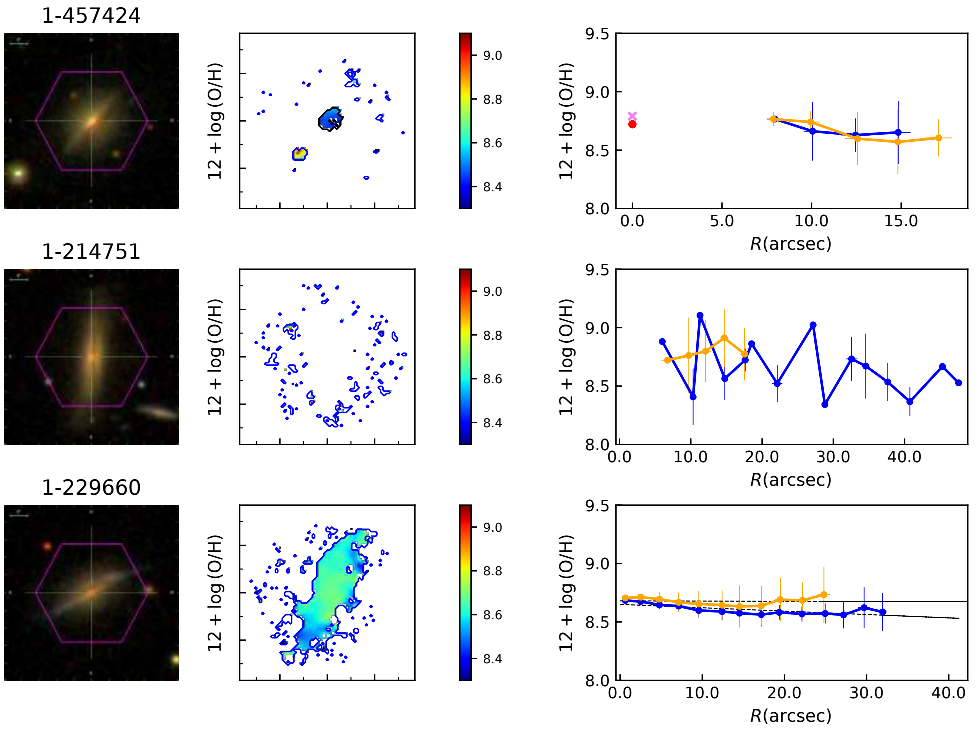


**Figure A75.** As Fig 3 but for the AGN host 1-457424.
